# Supplementary material for: Cayley graphs of order 30p are hamiltonian
Source: arXiv:1102.5156 ancillary file (2012-07-02)
Supplement: Supplementary file 1 [file 150.pdf]

# CAYLEY GRAPHS OF ORDER 150 ARE HAMILTONIAN

EBRAHIM GHADERPOUR AND DAVE WITTE MORRIS

Abstract. Suppose $G$ is a finite group of order 150, and $S$ is any generating set of $G$. We show there is a hamiltonian cycle in the corresponding Cayley graph $\mathrm{Cay}(G;S)$.

## A. Introduction

This is an (unpublished) appendix to [16]. In order to complete the proof of Proposition 2.10 of that paper, we establish the following result:

(A.1) **Proposition.** *If* $|G| = 150$*, then every connected Cayley graph on* $G$ *has a hamiltonian cycle.*

**Notation.** In this paper:

- $G$ is always a group of order 150,
- $S$ is a minimal generating set for $G$, and
- $P$ is a Sylow 5-subgroup of $G$, so $|P| = 25$.

**Outline of the proof of Proposition A.1.** We will first show that $P$ is a normal subgroup of $G$ (see Lemma B.1), and then note that the proof is easy if $P$ is cyclic (see Lemma B.2). Then two different cases will be considered:

§C: Assume $P$ is not cyclic, and $G/P$ is abelian.
§D: Assume $P$ is not cyclic, and $G/P$ is not abelian. □

*Acknowledgments.* This research was partially supported by grants from the Natural Sciences and Engineering Research Council of Canada.

## B. Preliminaries

(B.1) **Lemma.** *$P$ is a normal subgroup of $G$.*

**Proof.** Suppose $P \ntriangleleft G$. From Sylow's Theorems, we know that $N_G(P)$ has index 6 in $G$, so $P$ is self-normalizing. Therefore, $G$ has a normal 5-complement; i.e., a normal subgroup $H$ of order 6. Since no group of order 6 has an automorphism of order 5, we see that $P$ centralizes $H$, so $G = H \times P$. This contradicts our assumption that $P \ntriangleleft G$. □

(B.2) **Lemma.** *If $P$ is cyclic, then* $\mathrm{Cay}(G;S)$ *has a hamiltonian cycle.*

**Proof.** Every Sylow subgroup of $G$ is cyclic, so we may write $G = \mathbb{Z}_m \ltimes \mathbb{Z}_n$ with $\gcd(m,n) = 1$ [7, Thm. 9.4.3, p. 146]. Since $P$ is normal, we may assume $25 \mid n$. We may also assume $n \neq 25$, and $G' = \mathbb{Z}_n$, for otherwise Theorem 2.1 applies. Then $G = \mathbb{Z}_2 \ltimes \mathbb{Z}_{75}$ is dihedral, so Lemma 2.8 applies. □

*Date*: April 4, 2011.

## C. Assume $G/P$ is abelian

(C.1) **Proposition.** *If $P$ is a noncyclic, normal subgroup of $G$, and $G/P$ is abelian, then $\mathrm{Cay}(G;S)$ has a hamiltonian cycle.*

**Proof.** Note that, since $|P| = 25$, we have $P \cong \mathbb{Z}_5 \times \mathbb{Z}_5$. We may assume $G' = P$ (otherwise Theorem 2.1 applies).

**Case C1.** *Assume $\mathbb{Z}_2$ centralizes $P$.* Then

$$G = \mathbb{Z}_2 \times \big(\mathbb{Z}_3 \ltimes (\mathbb{Z}_5)^2\big) = \langle x \rangle \times \big(\langle y \rangle \ltimes \langle v_1, v_2 \rangle\big),$$

where $y$ acts via multiplication on the right by the matrix $\begin{bmatrix} 0 & 1 \\ -1 & -1 \end{bmatrix}$. Let $s \in S$, such that the projection of $s$ to $\mathbb{Z}_2$ is nontrivial. We may assume $s \notin \mathbb{Z}_2$ (otherwise Lemma 2.5(1) applies). Since $\mathbb{Z}_3$ acts irreducibly on $\mathbb{Z}_5 \times \mathbb{Z}_5$, this implies $\#S = 2$.

Let $^-$ be the natural homomorphism from $G$ to $\overline{G} = G/\mathbb{Z}_2$. From [10, Prop. 4.1], we know there is a hamiltonian cycle in $\mathrm{Cay}(\overline{G};S)$. Obviously, this hamiltonian cycle has odd length.

If $a$ and $b$ both have nontrivial projection to $\mathbb{Z}_2$, then the endpoint is nontrivial (since the hamiltonian cycle has odd length), so the Factor Group Lemma (2.2) provides a hamiltonian cycle in $G$.

So we may now assume $b$ projects trivially to $\mathbb{Z}_2$.

**Subcase C1.1.** *Assume $S \cap (\mathbb{Z}_2 \times P) = \emptyset$.* Then we may assume $\overline{bP} = \overline{aP}$ (by replacing $b$ with its inverse if necessary). Then an automorphism of $\overline{G}$ interchanges $\overline{a}$ with $\overline{b}$, so there is a hamiltonian cycle in $\mathrm{Cay}(\overline{G};\overline{S})$ with an odd number of occurrences of $\overline{a}$. So the Factor Group Lemma (2.2) provides a hamiltonian cycle in $G$.

**Subcase C1.2.** *Assume $a \in \mathbb{Z}_2 \times P$.* Then we may assume $a = xv_1$. Since $\langle a, b \rangle = G$, we know $b \notin \mathbb{Z}_2 \times P$. Then, since $b$ projects trivially to $\mathbb{Z}_2$, we may assume $b = y$ (perhaps after replacing $b$ with its inverse). A hamiltonian cycle is given on page 6.

**Subcase C1.3.** *Assume $S \cap (\mathbb{Z}_2 \times P) = \{b\}$.* Since $b$ projects trivially to $\mathbb{Z}_2$, we must have $b \in P$, so we may assume $b = v_1$. Also, since $a \notin \mathbb{Z}_2 \times P$, and $a$ projects nontrivially to $\mathbb{Z}_2$, we may assume $a = xy$ (perhaps after replacing $a$ with its inverse). A hamiltonian cycle is given on page 7.

**Case C2.** *Assume $\mathbb{Z}_3$ centralizes $P$.* Then $\mathbb{Z}_2$ must invert $P$. So $G = \mathbb{Z}_3 \times \big(\mathbb{Z}_2 \ltimes P\big)$, where $\mathbb{Z}_2$ inverts $P$. Some $c \in S$ has nontrivial projection to $\mathbb{Z}_3$. Then we may assume $c \in \mathbb{Z}_3 \times P$, for otherwise $c$ has order 2 in $G/\mathbb{Z}_3$, so Corollary 2.3 applies.

**Subcase C2.1.** *Assume $c$ is the only element of $S$ that belongs to $\mathbb{Z}_3 \times P$.* Then we may assume all of the other elements of $S$ belong to $\mathbb{Z}_2 \ltimes P$. And we may assume they all have order 2 (otherwise Lemma 2.5(3) applies. Since $S$ generates $G$, there must be at least two such elements; call them $a$ and $b$. Then $ab \in P$, so $\langle ab \rangle \triangleleft G$, so Corollary 2.3 applies.

**Subcase C2.2.** *Assume another element $b$ of $S$ belongs to $\mathbb{Z}_3 \times P$.* We may assume $b \equiv c \pmod{P}$, by replacing $b$ with its inverse if necessary. Then $\langle b^{-1}c \rangle \triangleleft G$, and $b \equiv c \pmod{\langle b^{-1}c \rangle}$, so Corollary 2.3 applies.

**Case C3.** *Assume $P$ is self-centralizing.* Then

$$G = (\mathbb{Z}_2 \times \mathbb{Z}_3) \ltimes (\mathbb{Z}_5)^2 = (\langle x \rangle \times \langle y \rangle) \ltimes P,$$

where $x$ inverts $P$, and $y$ acts via multiplication on the right by the matrix $\begin{bmatrix} 0 & 1 \\ -1 & -1 \end{bmatrix}$.

Let $^-$ be the natural homomorphism from $G$ to $G/P$.

**Subcase C3.1.** *Assume $\overline{S}$ contains an element of order* 6. Since $C_P(\overline{G})$ is trivial, we know this element also has order 6 in $G$, so we may assume it is the generator $xy$ of $\mathbb{Z}_2 \times \mathbb{Z}_3$, and either:

- $S = \{xy, (1,0)\}$: see hamiltonian cycle on page 8, or
- $S = \{xy, xy(1,0)\}$: see hamiltonian cycle on page 9, or
- $S = \{xy, x(1,0)\}$: see hamiltonian cycle on page 10, or
- $S = \{xy, y(1,0)\}$: see hamiltonian cycle on page 11.

**Subcase C3.2.** *Assume $\#S = 2$, and $\overline{S}$ has no element of order* 6. We may assume $S = \{xv, yv'\}$, for some $v, v' \in P$. By passing to a conjugate, we may assume $v = e$. Therefore, we may assume

$$S = \{x, y(1,0)\}.$$

A hamiltonian cycle is given on page 12.

**Subcase C3.3.** *Assume $\#S = 3$.* Choose $a, b \in S$, such that $\{a, b\}$ generates $\overline{G}$. Since $\langle a, b\rangle \neq G$, we may assume, by passing to a conjugate, that $\langle a, b\rangle = \mathbb{Z}_2 \times \mathbb{Z}_3$. Thus, we may assume $a = x$ and $b = y$. Since $S$ is minimal, its third element must belong to $P$. So we may assume $S = \{x, y, (1,0)\}$. A hamiltonian cycle is given on page 13. □

## D. Assume $G/P$ is not abelian

(D.1) **Proposition.** *If $P$ is a noncyclic, normal subgroup of $G$, and $G/P$ is not abelian, then* $\mathrm{Cay}(G;S)$ *has a hamiltonian cycle.*

**Proof.** We have $G = D_6 \ltimes P$. Write $D_6 = \langle\, f, t \mid f^2 = t^3 = (ft)^2 = e \,\rangle$.

**Case D1.** *Assume $t$ centralizes $P$, and $f$ inverts $P$.* Then $G = \mathbb{Z}_2 \ltimes (\mathbb{Z}_3 \times P)$, where $t$ inverts the abelian group $\mathbb{Z}_2 \ltimes (\mathbb{Z}_3 \times P)$. (In the terminology of [10, Defn. 2.21], $G$ is of *dihedral type.*) Since every subgroup of $\mathbb{Z}_3 \times P$ is normal, we may assume $S \cap (\mathbb{Z}_3 \times P) = \emptyset$ (otherwise Lemma 2.5(2) applies). Then, from the minimality of $S$, it is not difficult to see that $\#S \leq 3$. So the argument in [15] provides a hamiltonian cycle in $\mathrm{Cay}(G;S)$.

**Case D2.** *Assume $t$ centralizes $P$, and $f$ does not invert $P$.* Then $G = D_{6p} \times \mathbb{Z}_p$. Let $T$ be the group of rotations in $D_{6p}$.

Some element of $S$ projects to a reflection in $D_{6p}$. We may assume its projection to $\mathbb{Z}_p$ is trivial (otherwise Corollary 2.3 applies). Thus, by replacing it with a conjugate, we may assume $f \in S$.

Some element $c$ of $S$ projects nontrivially to $\mathbb{Z}_p$. From the preceding paragraph, we may assume $c \in T \times \mathbb{Z}_p$; write $c = t_0 z$ with $t_0 \in T$ and $\langle z\rangle = \mathbb{Z}_p$. Note that $t_0$ is nontrivial (otherwise Lemma 2.5(1) applies).

**Subcase D2.1.** *Assume $\langle t_0\rangle \neq T$.* Then $\langle f, c\rangle \neq G$, so there exists $s \in S \smallsetminus \{f, c\}$. We may assume $s \notin T \times \mathbb{Z}_p$; otherwise Lemma 2.6 applies. Thus, the projection of $s$ to $D_{6p}$ is a reflection, so we may assume $s \in D_{6p}$ (otherwise Corollary 2.3 applies). Furthermore, we may assume $|fs|$ is not prime (otherwise Corollary 2.3 applies), so $|fs| = 3p$. Then $(f, c^{p-1}, s, c^{p-1})^{3p}$ is a hamiltonian cycle in $\mathrm{Cay}(G;S)$.

**Subcase D2.2.** *Assume $\langle t_0\rangle = T$.* Then $(c^{3p-1}, f)^2$ is a hamiltonian cycle in $\mathrm{Cay}(G/\mathbb{Z}_p;S)$. Its endpoint in $G$ is

$$(c^{3p-1}f)^2 = \big((t_0 z)^{3p-1} f\big)^2 = z^{2(3p-1)},$$

which generates $\mathbb{Z}_p$, so the Factor Group Lemma (2.2) provides a hamiltonian cycle in $\mathrm{Cay}(G;S)$.

**Case D3.** *Assume $t$ does not centralize $P$.* Now, since $f$ inverts $t$, it is clear that the action of $f$ is not in the center of $\mathrm{Aut}(P)$; so $f$ neither centralizes nor inverts $P$. Then, since $f^2 = e$, we may choose a basis so that

$$f \text{ acts on } P \text{ via multiplication on the right by the matrix } J = \begin{bmatrix} 1 & 0 \\ 0 & -1 \end{bmatrix}.$$

Now, let $[\alpha_1, \alpha_2] = [1,0]^t$. Multiplying the second basis vector by a scalar, we may assume $\alpha_2 = 1$. Since $f$ inverts $t$, we must have $[\alpha_1, -1]^t = [1,0]$. Then, since $t^3 = e$, we must have $[\alpha_1, 1]^t = [\alpha_1, -1]$. Solving the resulting linear equations leads to the conclusion that

$$t \text{ acts on } P \text{ via multiplication on the right by the matrix } C = \begin{bmatrix} -1/2 & 1 \\ -3/4 & -1/2 \end{bmatrix} = \begin{bmatrix} 2 & 1 \\ 3 & 2 \end{bmatrix}$$

(since the coordinates of vectors in $P = (\mathbb{Z}_5)^2$ are taken modulo 5).

Now we find the possible generating sets. Let $\overline{\phantom{x}}$ be the natural homomorphism from $G$ to $G/P$. Since $G/P \cong D_6$, we may choose $a, b \in S$, such that $\{a, b\}$ generates $G/P$. Then, since $t$ acts irreducibly on $P$, it is clear that $\#S \leq 3$.

Note that

$$\begin{aligned} \begin{bmatrix} 1 & 0 \end{bmatrix} J &= \begin{bmatrix} 1 & 0 \end{bmatrix}, \\ \begin{bmatrix} 0 & 1 \end{bmatrix} J &= -\begin{bmatrix} 0 & 1 \end{bmatrix}, \\ \begin{bmatrix} 1 & 2 \end{bmatrix} JC &= \begin{bmatrix} 1 & 2 \end{bmatrix}, \end{aligned}$$

and

$$\begin{bmatrix} 1 & 1 \end{bmatrix} JC = -\begin{bmatrix} 1 & 1 \end{bmatrix}.$$

We may assume $\overline{a} = f$.

**Subcase D3.1.** *Assume $\#S = 2$.*

**Subsubcase D3.1.1.** *Assume $\overline{b}$ is a rotation.* By passing to a conjugate, we may assume $b = t$.

We have $a = fv$, for some nontrivial $v \in P$. After multiplying $v$ by a nonzero scalar, and perhaps conjugating by $f$, we may assume

$$v \in \{(1,0), (1,1), (1,2), (0,1)\}.$$

Hamiltonian cycles for the resulting generating sets can be found on pages 14, 15, 16, and 17.

**Subsubcase D3.1.2.** *Assume $\overline{b}$ is a reflection.* We may assume $b = ftv_2$, for some $v_2 \in P$. Replacing $a$ by a conjugate, we may assume $a = fv_1$, where $v_1 \in C_P(f)$. Then, conjugating by an element of $C_P(a)$, we may assume $v_2 \in C_P(b)$. Since $\langle a, b \rangle = G$, we know that $v_1$ and $v_2$ are not both trivial, so we may assume $v_1 \neq (0,0)$. Then, multiplying by a scalar, we may assume $v_1 = (1,0)$. And $v_2$ is a scalar multiple of $(1,2)$. We may assume the scalar is in $\{0,1,2\}$, by replacing $b$ with its inverse if necessary. So

$$S = \{f(1,0), ft(\lambda, 2\lambda)\}, \text{ for some } \lambda \in \{0,1,2\}.$$

Hamiltonian cycles for the three values of $\lambda$ are given on pages 18, 19, and 20.

**Subcase D3.2.** *Assume $\#S = 3$.* Passing to a conjugate, we may assume $\langle a, b \rangle = D_6$, so we may assume $b \in \{t, ft\}$.

Let $c$ be the third element of $S$, so $c = gv$, for some $g \in D_6$ and some nontrivial $v \in P$.

**Subsubcase D3.2.1.** *Assume $b = t$.* Since $\langle t, c\rangle = \langle b, c\rangle \neq G$, we must have $g \in \langle t\rangle$; so we may assume $g \in \{e, t\}$.

**Subsubsubcase D3.2.1.1.** *Assume $g = e$.* Then $S = \{f, t, v\}$, for some nontrivial $v \in (\mathbb{Z}_5)^2$.

- Suppose $v$ is not an eigenvector for $f$. Then $|\langle f, v\rangle| = 50$, and we know that $\mathrm{Cay}\big(\langle f, v\rangle; \{f, v\}\big)$ is hamiltonian [10, Cor. 2.24]. So it has a hamiltonian path $L$ from $e$ to $v$. Then $(L, t)^3$ is a hamiltonian cycle in $\mathrm{Cay}(G; S)$. (The endpoint of this walk is $(vt)^3$, which is trivial, because $t$ has trivial centralizer in $P$.)
- Suppose $v$ is an eigenvector for $f$. Then there exists $\epsilon \in \{\pm 1\}$ with $v^f = v^\epsilon$ Note that $|\langle t, v\rangle| = 75$, and we know that $\mathrm{Cay}\big(\langle t, v\rangle; \{t, v\}\big)$ is hamiltonian [10, Prop. 4.1]. So it has a hamiltonian path $L$ from $e$ to $v$. Then $(L, f, L^{-\epsilon}, f)$ is a hamiltonian cycle in $\mathrm{Cay}(G; S)$. (The endpoint of this walk is $v f v^{-\epsilon} f$, which is trivial, because $(v^\epsilon)^f = v$.)

**Subsubsubcase D3.2.1.2.** *Assume $g = t$.* Then

$$c\, c^a = (tv)\,(tv)^f = (tv)(t^{-1}v^f) = v^{t^2} v^f,$$

so, since $\langle a, c\rangle \neq G$, we must have $v^{t^2} v^f = e$, so $v^{ft} = v^{-1}$. Therefore, we may assume (by passing to a scalar multiple) that $v = (1, 1)$. So $S = \{f, t, t(1, 1)\}$. A hamiltonian cycle is given on page 21.

**Subsubcase D3.2.2.** *Assume $b = ft$.* If $\overline{c}$ is nontrivial, we may assume it is a reflection (otherwise, Subsubcase D3.2.1 applies with $c$ in the place of $b$). And if $\overline{c} \in \{a, b\}$, there is no harm in assuming $\overline{c} = a$, since we may interchange $a$ and $b$. So either:

- $S = \{f, ft, v\}$, for some nontrivial $v \in (\mathbb{Z}_5)^2$, or
- $S = \{f, ft, fv\}$, for some nontrivial $v \in (\mathbb{Z}_5)^2$, or
- $S = \{f, ft, ft^2 v\}$, for some nontrivial $v \in (\mathbb{Z}_5)^2$.

**Subsubsubcase D3.2.2.1.** *Assume $S = \{f, ft, v\}$.* Since $f$ and $ft$ do not have any common eigenvectors, we may assume $v$ is not an eigenvector for $f$ (by applying an automorphism that interchanges $f$ and $ft$ if necessary). Then $|\langle f, c\rangle| = 50$, and we know that $\mathrm{Cay}\big(\langle f, c\rangle; \{f, c\}\big)$ is hamiltonian [10, Cor. 2.24]. So it has a hamiltonian path $L$ from $e$ to $f$. Then $(L, ft)^3$ is a hamiltonian cycle in $\mathrm{Cay}(G; S)$. (The endpoint of this walk is $(f \cdot ft)^3 = t^3 = e$.)

**Subsubsubcase D3.2.2.2.** *Assume $S = \{f, ft, fv\}$.* Since $\langle ft, fv\rangle \neq G$, we must have $(fv)^2 = e$, so $v^f = v^{-1}$. Therefore (by passing to a scalar multiple) we may assume $v = (0, 1)$. A hamiltonian cycle is given on page 22.

**Subsubsubcase D3.2.2.3.** *Assume $S = \{f, ft, ft^2 v\}$.* Since $\langle f, ft^2 v\rangle \neq G$, we must have $(ft^2 v)^2 = e$, so $v^{ft^2} = v^{-1}$. And note that $ft^2$ acts via multiplication on the right by

$$JC^2 = \begin{bmatrix} 2 & 4 \\ 3 & 3 \end{bmatrix}.$$

Therefore (by passing to a scalar multiple) we may assume $v = (1, -1)$. A hamiltonian cycle is given on page 23. □

$$S = \{xv_1, y\} \text{ in } G = \mathbb{Z}_2 \times \big(\mathbb{Z}_3 \ltimes (\mathbb{Z}_5)^2\big)$$

$$\begin{array}{ccccccccccc}
\overline{(0,0)} & \xrightarrow{a^{-1}} & \overline{x(4,0)} & \xrightarrow{a^{-1}} & \overline{(3,0)} & \xrightarrow{a^{-1}} & \overline{x(2,0)} & \xrightarrow{a^{-1}} & \overline{(1,0)} & \xrightarrow{a^{-1}} & \overline{x(0,0)} \\
& \xrightarrow{a^{-1}} & \overline{(4,0)} & \xrightarrow{b} & \overline{y(0,4)} & \xrightarrow{a} & \overline{xy(1,4)} & \xrightarrow{b^{-1}} & \overline{x(3,4)} & \xrightarrow{a^{-1}} & \overline{(2,4)} \\
& \xrightarrow{a^{-1}} & \overline{x(1,4)} & \xrightarrow{a^{-1}} & \overline{(0,4)} & \xrightarrow{a^{-1}} & \overline{x(4,4)} & \xrightarrow{a^{-1}} & \overline{(3,4)} & \xrightarrow{a^{-1}} & \overline{x(2,4)} \\
& \xrightarrow{a^{-1}} & \overline{(1,4)} & \xrightarrow{a^{-1}} & \overline{x(0,4)} & \xrightarrow{a^{-1}} & \overline{(4,4)} & \xrightarrow{b} & \overline{y(1,0)} & \xrightarrow{a} & \overline{xy(2,0)} \\
& \xrightarrow{b^{-1}} & \overline{x(3,3)} & \xrightarrow{a^{-1}} & \overline{(2,3)} & \xrightarrow{a^{-1}} & \overline{x(1,3)} & \xrightarrow{a^{-1}} & \overline{(0,3)} & \xrightarrow{a^{-1}} & \overline{x(4,3)} \\
& \xrightarrow{a^{-1}} & \overline{(3,3)} & \xrightarrow{a^{-1}} & \overline{x(2,3)} & \xrightarrow{a^{-1}} & \overline{(1,3)} & \xrightarrow{a^{-1}} & \overline{x(0,3)} & \xrightarrow{a^{-1}} & \overline{(4,3)} \\
& \xrightarrow{b} & \overline{y(2,1)} & \xrightarrow{a^{-1}} & \overline{xy(1,1)} & \xrightarrow{a^{-1}} & \overline{y(0,1)} & \xrightarrow{a^{-1}} & \overline{xy(4,1)} & \xrightarrow{a^{-1}} & \overline{y(3,1)} \\
& \xrightarrow{a^{-1}} & \overline{xy(2,1)} & \xrightarrow{a^{-1}} & \overline{y(1,1)} & \xrightarrow{a^{-1}} & \overline{xy(0,1)} & \xrightarrow{a^{-1}} & \overline{y(4,1)} & \xrightarrow{b} & \overline{y^2(4,3)} \\
& \xrightarrow{a} & \overline{xy^2(0,3)} & \xrightarrow{b^{-1}} & \overline{xy(3,0)} & \xrightarrow{a^{-1}} & \overline{y(2,0)} & \xrightarrow{a^{-1}} & \overline{xy(1,0)} & \xrightarrow{a^{-1}} & \overline{y(0,0)} \\
& \xrightarrow{a^{-1}} & \overline{xy(4,0)} & \xrightarrow{a^{-1}} & \overline{y(3,0)} & \xrightarrow{b} & \overline{y^2(0,3)} & \xrightarrow{a^{-1}} & \overline{xy^2(4,3)} & \xrightarrow{a^{-1}} & \overline{y^2(3,3)} \\
& \xrightarrow{a^{-1}} & \overline{xy^2(2,3)} & \xrightarrow{a^{-1}} & \overline{y^2(1,3)} & \xrightarrow{b^{-1}} & \overline{y(2,4)} & \xrightarrow{a} & \overline{xy(3,4)} & \xrightarrow{b} & \overline{xy^2(1,4)} \\
& \xrightarrow{a} & \overline{y^2(2,4)} & \xrightarrow{a} & \overline{xy^2(3,4)} & \xrightarrow{a} & \overline{y^2(4,4)} & \xrightarrow{a} & \overline{xy^2(0,4)} & \xrightarrow{a} & \overline{y^2(1,4)} \\
& \xrightarrow{b^{-1}} & \overline{y(3,4)} & \xrightarrow{a} & \overline{xy(4,4)} & \xrightarrow{b} & \overline{xy^2(1,0)} & \xrightarrow{a^{-1}} & \overline{y^2(0,0)} & \xrightarrow{a^{-1}} & \overline{xy^2(4,0)} \\
& \xrightarrow{a^{-1}} & \overline{y^2(3,0)} & \xrightarrow{b^{-1}} & \overline{y(2,2)} & \xrightarrow{a^{-1}} & \overline{xy(1,2)} & \xrightarrow{a^{-1}} & \overline{y(0,2)} & \xrightarrow{a^{-1}} & \overline{xy(4,2)} \\
& \xrightarrow{b^{-1}} & \overline{x(3,1)} & \xrightarrow{a^{-1}} & \overline{(2,1)} & \xrightarrow{a^{-1}} & \overline{x(1,1)} & \xrightarrow{a^{-1}} & \overline{(0,1)} & \xrightarrow{a^{-1}} & \overline{x(4,1)} \\
& \xrightarrow{a^{-1}} & \overline{(3,1)} & \xrightarrow{a^{-1}} & \overline{x(2,1)} & \xrightarrow{a^{-1}} & \overline{(1,1)} & \xrightarrow{a^{-1}} & \overline{x(0,1)} & \xrightarrow{a^{-1}} & \overline{(4,1)} \\
& \xrightarrow{b} & \overline{y(4,3)} & \xrightarrow{b} & \overline{y^2(2,1)} & \xrightarrow{a^{-1}} & \overline{xy^2(1,1)} & \xrightarrow{a^{-1}} & \overline{y^2(0,1)} & \xrightarrow{a^{-1}} & \overline{xy^2(4,1)} \\
& \xrightarrow{a^{-1}} & \overline{y^2(3,1)} & \xrightarrow{a^{-1}} & \overline{xy^2(2,1)} & \xrightarrow{a^{-1}} & \overline{y^2(1,1)} & \xrightarrow{a^{-1}} & \overline{xy^2(0,1)} & \xrightarrow{a^{-1}} & \overline{y^2(4,1)} \\
& \xrightarrow{a^{-1}} & \overline{xy^2(3,1)} & \xrightarrow{b^{-1}} & \overline{xy(3,2)} & \xrightarrow{a} & \overline{y(4,2)} & \xrightarrow{b} & \overline{y^2(3,2)} & \xrightarrow{a^{-1}} & \overline{xy^2(2,2)} \\
& \xrightarrow{a^{-1}} & \overline{y^2(1,2)} & \xrightarrow{a^{-1}} & \overline{xy^2(0,2)} & \xrightarrow{a^{-1}} & \overline{y^2(4,2)} & \xrightarrow{a^{-1}} & \overline{xy^2(3,2)} & \xrightarrow{a^{-1}} & \overline{y^2(2,2)} \\
& \xrightarrow{a^{-1}} & \overline{xy^2(1,2)} & \xrightarrow{a^{-1}} & \overline{y^2(0,2)} & \xrightarrow{a^{-1}} & \overline{xy^2(4,2)} & \xrightarrow{b^{-1}} & \overline{xy(3,1)} & \xrightarrow{b^{-1}} & \overline{x(3,2)} \\
& \xrightarrow{a^{-1}} & \overline{(2,2)} & \xrightarrow{a^{-1}} & \overline{x(1,2)} & \xrightarrow{a^{-1}} & \overline{(0,2)} & \xrightarrow{a^{-1}} & \overline{x(4,2)} & \xrightarrow{a^{-1}} & \overline{(3,2)} \\
& \xrightarrow{a^{-1}} & \overline{x(2,2)} & \xrightarrow{a^{-1}} & \overline{(1,2)} & \xrightarrow{a^{-1}} & \overline{x(0,2)} & \xrightarrow{a^{-1}} & \overline{(4,2)} & \xrightarrow{b} & \overline{y(3,2)} \\
& \xrightarrow{a^{-1}} & \overline{xy(2,2)} & \xrightarrow{a^{-1}} & \overline{y(1,2)} & \xrightarrow{a^{-1}} & \overline{xy(0,2)} & \xrightarrow{b} & \overline{xy^2(3,3)} & \xrightarrow{a^{-1}} & \overline{y^2(2,3)} \\
& \xrightarrow{a^{-1}} & \overline{xy^2(1,3)} & \xrightarrow{b^{-1}} & \overline{xy(2,4)} & \xrightarrow{a^{-1}} & \overline{y(1,4)} & \xrightarrow{a^{-1}} & \overline{xy(0,4)} & \xrightarrow{a^{-1}} & \overline{y(4,4)} \\
& \xrightarrow{b} & \overline{y^2(1,0)} & \xrightarrow{a} & \overline{xy^2(2,0)} & \xrightarrow{b^{-1}} & \overline{xy(3,3)} & \xrightarrow{a^{-1}} & \overline{y(2,3)} & \xrightarrow{a^{-1}} & \overline{xy(1,3)} \\
& \xrightarrow{a^{-1}} & \overline{y(0,3)} & \xrightarrow{a^{-1}} & \overline{xy(4,3)} & \xrightarrow{a^{-1}} & \overline{y(3,3)} & \xrightarrow{b} & \overline{y^2(2,0)} & \xrightarrow{a} & \overline{xy^2(3,0)} \\
& \xrightarrow{a} & \overline{y^2(4,0)} & \xrightarrow{a} & \overline{xy^2(0,0)} & \xrightarrow{b^{-1}} & \overline{xy(0,0)} & \xrightarrow{a^{-1}} & \overline{y(4,0)} & \xrightarrow{b} & \overline{y^2(0,4)} \\
& \xrightarrow{a^{-1}} & \overline{xy^2(4,4)} & \xrightarrow{a^{-1}} & \overline{y^2(3,4)} & \xrightarrow{a^{-1}} & \overline{xy^2(2,4)} & \xrightarrow{b^{-1}} & \overline{xy(2,3)} & \xrightarrow{a^{-1}} & \overline{y(1,3)} \\
& \xrightarrow{a^{-1}} & \overline{xy(0,3)} & \xrightarrow{b^{-1}} & \overline{x(3,0)} & \xrightarrow{a^{-1}} & \overline{(2,0)} & \xrightarrow{a^{-1}} & \overline{x(1,0)} & \xrightarrow{a^{-1}} & \overline{(0,0)}
\end{array}$$

$$S = \{xy, v_1\} \text{ in } G = \mathbb{Z}_2 \times \big(\mathbb{Z}_3 \ltimes (\mathbb{Z}_5)^2\big)$$

$$
\begin{array}{lllllllllll}
\overline{(0,0)} & \xrightarrow{a^{-1}} & \overline{xy^2(0,0)} & \xrightarrow{a^{-1}} & \overline{y(0,0)} & \xrightarrow{a^{-1}} & \overline{x(0,0)} & \xrightarrow{a^{-1}} & \overline{y^2(0,0)} & \xrightarrow{b} & \overline{y^2(1,0)} \\
 & \xrightarrow{a} & \overline{x(0,1)} & \xrightarrow{a} & \overline{y(4,4)} & \xrightarrow{a} & \overline{xy^2(1,0)} & \xrightarrow{a} & \overline{(0,1)} & \xrightarrow{a} & \overline{xy(4,4)} \\
 & \xrightarrow{b^{-1}} & \overline{xy(3,4)} & \xrightarrow{a^{-1}} & \overline{(1,2)} & \xrightarrow{a^{-1}} & \overline{xy^2(1,4)} & \xrightarrow{a^{-1}} & \overline{y(3,4)} & \xrightarrow{a^{-1}} & \overline{x(1,2)} \\
 & \xrightarrow{b^{-1}} & \overline{x(0,2)} & \xrightarrow{a} & \overline{y(3,3)} & \xrightarrow{a} & \overline{xy^2(2,0)} & \xrightarrow{a} & \overline{(0,2)} & \xrightarrow{a} & \overline{xy(3,3)} \\
 & \xrightarrow{a} & \overline{y^2(2,0)} & \xrightarrow{b} & \overline{y^2(3,0)} & \xrightarrow{b} & \overline{y^2(4,0)} & \xrightarrow{a^{-1}} & \overline{xy(1,1)} & \xrightarrow{a^{-1}} & \overline{(0,4)} \\
 & \xrightarrow{a^{-1}} & \overline{xy^2(4,0)} & \xrightarrow{a^{-1}} & \overline{y(1,1)} & \xrightarrow{a^{-1}} & \overline{x(0,4)} & \xrightarrow{b} & \overline{x(1,4)} & \xrightarrow{a} & \overline{y(1,2)} \\
 & \xrightarrow{a} & \overline{xy^2(3,4)} & \xrightarrow{a} & \overline{(1,4)} & \xrightarrow{a} & \overline{xy(1,2)} & \xrightarrow{a} & \overline{y^2(3,4)} & \xrightarrow{b} & \overline{y^2(4,4)} \\
 & \xrightarrow{a^{-1}} & \overline{xy(0,1)} & \xrightarrow{a^{-1}} & \overline{(1,0)} & \xrightarrow{a^{-1}} & \overline{xy^2(4,4)} & \xrightarrow{a^{-1}} & \overline{y(0,1)} & \xrightarrow{a^{-1}} & \overline{x(1,0)} \\
 & \xrightarrow{b} & \overline{x(2,0)} & \xrightarrow{a} & \overline{y(0,2)} & \xrightarrow{a} & \overline{xy^2(3,3)} & \xrightarrow{a} & \overline{(2,0)} & \xrightarrow{a} & \overline{xy(0,2)} \\
 & \xrightarrow{b^{-1}} & \overline{xy(4,2)} & \xrightarrow{a^{-1}} & \overline{(3,1)} & \xrightarrow{a^{-1}} & \overline{xy^2(3,2)} & \xrightarrow{a^{-1}} & \overline{y(4,2)} & \xrightarrow{a^{-1}} & \overline{x(3,1)} \\
 & \xrightarrow{b} & \overline{x(4,1)} & \xrightarrow{a} & \overline{y(4,3)} & \xrightarrow{a} & \overline{xy^2(2,1)} & \xrightarrow{a} & \overline{(4,1)} & \xrightarrow{a} & \overline{xy(4,3)} \\
 & \xrightarrow{a} & \overline{y^2(2,1)} & \xrightarrow{b} & \overline{y^2(3,1)} & \xrightarrow{b} & \overline{y^2(4,1)} & \xrightarrow{a^{-1}} & \overline{xy(2,1)} & \xrightarrow{a^{-1}} & \overline{(4,3)} \\
 & \xrightarrow{a^{-1}} & \overline{xy^2(4,1)} & \xrightarrow{a^{-1}} & \overline{y(2,1)} & \xrightarrow{a^{-1}} & \overline{x(4,3)} & \xrightarrow{b} & \overline{x(0,3)} & \xrightarrow{a} & \overline{y(2,2)} \\
 & \xrightarrow{a} & \overline{xy^2(3,0)} & \xrightarrow{a} & \overline{(0,3)} & \xrightarrow{a} & \overline{xy(2,2)} & \xrightarrow{b} & \overline{xy(3,2)} & \xrightarrow{a^{-1}} & \overline{(4,2)} \\
 & \xrightarrow{a^{-1}} & \overline{xy^2(3,1)} & \xrightarrow{a^{-1}} & \overline{y(3,2)} & \xrightarrow{a^{-1}} & \overline{x(4,2)} & \xrightarrow{b^{-1}} & \overline{x(3,2)} & \xrightarrow{a} & \overline{y(3,1)} \\
 & \xrightarrow{a} & \overline{xy^2(4,2)} & \xrightarrow{a} & \overline{(3,2)} & \xrightarrow{a} & \overline{xy(3,1)} & \xrightarrow{a} & \overline{y^2(4,2)} & \xrightarrow{b^{-1}} & \overline{y^2(3,2)} \\
 & \xrightarrow{b^{-1}} & \overline{y^2(2,2)} & \xrightarrow{a} & \overline{x(3,0)} & \xrightarrow{a} & \overline{y(0,3)} & \xrightarrow{a} & \overline{xy^2(2,2)} & \xrightarrow{a} & \overline{(3,0)} \\
 & \xrightarrow{a} & \overline{xy(0,3)} & \xrightarrow{b} & \overline{xy(1,3)} & \xrightarrow{a^{-1}} & \overline{(2,4)} & \xrightarrow{a^{-1}} & \overline{xy^2(2,3)} & \xrightarrow{a^{-1}} & \overline{y(1,3)} \\
 & \xrightarrow{a^{-1}} & \overline{x(2,4)} & \xrightarrow{a^{-1}} & \overline{y^2(2,3)} & \xrightarrow{b} & \overline{y^2(3,3)} & \xrightarrow{b} & \overline{y^2(4,3)} & \xrightarrow{a^{-1}} & \overline{xy(4,1)} \\
 & \xrightarrow{a^{-1}} & \overline{(2,1)} & \xrightarrow{a^{-1}} & \overline{xy^2(4,3)} & \xrightarrow{a^{-1}} & \overline{y(4,1)} & \xrightarrow{a^{-1}} & \overline{x(2,1)} & \xrightarrow{b^{-1}} & \overline{x(1,1)} \\
 & \xrightarrow{a} & \overline{y(4,0)} & \xrightarrow{a} & \overline{xy^2(0,4)} & \xrightarrow{a} & \overline{(1,1)} & \xrightarrow{a} & \overline{xy(4,0)} & \xrightarrow{a} & \overline{y^2(0,4)} \\
 & \xrightarrow{b} & \overline{y^2(1,4)} & \xrightarrow{b} & \overline{y^2(2,4)} & \xrightarrow{a^{-1}} & \overline{xy(2,3)} & \xrightarrow{a^{-1}} & \overline{(1,3)} & \xrightarrow{a^{-1}} & \overline{xy^2(2,4)} \\
 & \xrightarrow{a^{-1}} & \overline{y(2,3)} & \xrightarrow{a^{-1}} & \overline{x(1,3)} & \xrightarrow{b} & \overline{x(2,3)} & \xrightarrow{a} & \overline{y(2,4)} & \xrightarrow{a} & \overline{xy^2(1,3)} \\
 & \xrightarrow{a} & \overline{(2,3)} & \xrightarrow{a} & \overline{xy(2,4)} & \xrightarrow{a} & \overline{y^2(1,3)} & \xrightarrow{b^{-1}} & \overline{y^2(0,3)} & \xrightarrow{a} & \overline{x(2,2)} \\
 & \xrightarrow{a} & \overline{y(3,0)} & \xrightarrow{a} & \overline{xy^2(0,3)} & \xrightarrow{a} & \overline{(2,2)} & \xrightarrow{a} & \overline{xy(3,0)} & \xrightarrow{b^{-1}} & \overline{xy(2,0)} \\
 & \xrightarrow{a^{-1}} & \overline{(3,3)} & \xrightarrow{a^{-1}} & \overline{xy^2(0,2)} & \xrightarrow{a^{-1}} & \overline{y(2,0)} & \xrightarrow{a^{-1}} & \overline{x(3,3)} & \xrightarrow{a^{-1}} & \overline{y^2(0,2)} \\
 & \xrightarrow{b} & \overline{y^2(1,2)} & \xrightarrow{a} & \overline{x(3,4)} & \xrightarrow{a} & \overline{y(1,4)} & \xrightarrow{a} & \overline{xy^2(1,2)} & \xrightarrow{a} & \overline{(3,4)} \\
 & \xrightarrow{a} & \overline{xy(1,4)} & \xrightarrow{b^{-1}} & \overline{xy(0,4)} & \xrightarrow{a^{-1}} & \overline{(4,0)} & \xrightarrow{a^{-1}} & \overline{xy^2(1,1)} & \xrightarrow{a^{-1}} & \overline{y(0,4)} \\
 & \xrightarrow{a^{-1}} & \overline{x(4,0)} & \xrightarrow{a^{-1}} & \overline{y^2(1,1)} & \xrightarrow{b^{-1}} & \overline{y^2(0,1)} & \xrightarrow{a} & \overline{x(4,4)} & \xrightarrow{a} & \overline{y(1,0)} \\
 & \xrightarrow{a} & \overline{xy^2(0,1)} & \xrightarrow{a} & \overline{(4,4)} & \xrightarrow{a} & \overline{xy(1,0)} & \xrightarrow{b^{-1}} & \overline{xy(0,0)} & \xrightarrow{a^{-1}} & \overline{(0,0)}
\end{array}
$$

$$S = \{xy, (1,0)\} \text{ in } G = (\mathbb{Z}_2 \times \mathbb{Z}_3) \ltimes (\mathbb{Z}_5)^2$$

$$\overline{e} \xrightarrow{b^{-1}} \overline{(4,0)} \xrightarrow{a} \overline{xy(0,1)} \xrightarrow{b} \overline{xy(1,1)} \xrightarrow{b} \overline{xy(2,1)} \xrightarrow{b} \overline{xy(3,1)}$$
$$\xrightarrow{b} \overline{xy(4,1)} \xrightarrow{a^{-1}} \overline{(3,4)} \xrightarrow{b^{-1}} \overline{(2,4)} \xrightarrow{b^{-1}} \overline{(1,4)} \xrightarrow{b^{-1}} \overline{(0,4)}$$
$$\xrightarrow{b^{-1}} \overline{(4,4)} \xrightarrow{a} \overline{xy(4,0)} \xrightarrow{b} \overline{xy(0,0)} \xrightarrow{b} \overline{xy(1,0)} \xrightarrow{b} \overline{xy(2,0)}$$
$$\xrightarrow{b} \overline{xy(3,0)} \xrightarrow{a^{-1}} \overline{(3,3)} \xrightarrow{b^{-1}} \overline{(2,3)} \xrightarrow{b^{-1}} \overline{(1,3)} \xrightarrow{b^{-1}} \overline{(0,3)}$$
$$\xrightarrow{b^{-1}} \overline{(4,3)} \xrightarrow{a} \overline{xy(3,4)} \xrightarrow{b} \overline{xy(4,4)} \xrightarrow{b} \overline{xy(0,4)} \xrightarrow{b} \overline{xy(1,4)}$$
$$\xrightarrow{a} \overline{y^2(4,3)} \xrightarrow{b} \overline{y^2(0,3)} \xrightarrow{b} \overline{y^2(1,3)} \xrightarrow{b} \overline{y^2(2,3)} \xrightarrow{b} \overline{y^2(3,3)}$$
$$\xrightarrow{a} \overline{x(3,0)} \xrightarrow{b^{-1}} \overline{x(2,0)} \xrightarrow{b^{-1}} \overline{x(1,0)} \xrightarrow{b^{-1}} \overline{x(0,0)} \xrightarrow{b^{-1}} \overline{x(4,0)}$$
$$\xrightarrow{a^{-1}} \overline{y^2(4,4)} \xrightarrow{b} \overline{y^2(0,4)} \xrightarrow{b} \overline{y^2(1,4)} \xrightarrow{b} \overline{y^2(2,4)} \xrightarrow{b} \overline{y^2(3,4)}$$
$$\xrightarrow{a} \overline{x(4,1)} \xrightarrow{b^{-1}} \overline{x(3,1)} \xrightarrow{b^{-1}} \overline{x(2,1)} \xrightarrow{b^{-1}} \overline{x(1,1)} \xrightarrow{b^{-1}} \overline{x(0,1)}$$
$$\xrightarrow{a^{-1}} \overline{y^2(4,0)} \xrightarrow{b} \overline{y^2(0,0)} \xrightarrow{b} \overline{y^2(1,0)} \xrightarrow{b} \overline{y^2(2,0)} \xrightarrow{a} \overline{x(0,3)}$$
$$\xrightarrow{b} \overline{x(1,3)} \xrightarrow{b} \overline{x(2,3)} \xrightarrow{b} \overline{x(3,3)} \xrightarrow{b} \overline{x(4,3)} \xrightarrow{a} \overline{y(3,4)}$$
$$\xrightarrow{a} \overline{xy^2(4,1)} \xrightarrow{b^{-1}} \overline{xy^2(3,1)} \xrightarrow{b^{-1}} \overline{xy^2(2,1)} \xrightarrow{b^{-1}} \overline{xy^2(1,1)} \xrightarrow{b^{-1}} \overline{xy^2(0,1)}$$
$$\xrightarrow{a^{-1}} \overline{y(4,0)} \xrightarrow{b} \overline{y(0,0)} \xrightarrow{b} \overline{y(1,0)} \xrightarrow{b} \overline{y(2,0)} \xrightarrow{b} \overline{y(3,0)}$$
$$\xrightarrow{a} \overline{xy^2(0,2)} \xrightarrow{b} \overline{xy^2(1,2)} \xrightarrow{b} \overline{xy^2(2,2)} \xrightarrow{b} \overline{xy^2(3,2)} \xrightarrow{b} \overline{xy^2(4,2)}$$
$$\xrightarrow{a^{-1}} \overline{y(2,4)} \xrightarrow{b^{-1}} \overline{y(1,4)} \xrightarrow{b^{-1}} \overline{y(0,4)} \xrightarrow{b^{-1}} \overline{y(4,4)} \xrightarrow{a} \overline{xy^2(4,0)}$$
$$\xrightarrow{b} \overline{xy^2(0,0)} \xrightarrow{b} \overline{xy^2(1,0)} \xrightarrow{b} \overline{xy^2(2,0)} \xrightarrow{b} \overline{xy^2(3,0)} \xrightarrow{a^{-1}} \overline{y(3,3)}$$
$$\xrightarrow{b^{-1}} \overline{y(2,3)} \xrightarrow{b^{-1}} \overline{y(1,3)} \xrightarrow{b^{-1}} \overline{y(0,3)} \xrightarrow{b^{-1}} \overline{y(4,3)} \xrightarrow{a} \overline{xy^2(3,4)}$$
$$\xrightarrow{b} \overline{xy^2(4,4)} \xrightarrow{b} \overline{xy^2(0,4)} \xrightarrow{b} \overline{xy^2(1,4)} \xrightarrow{b} \overline{xy^2(2,4)} \xrightarrow{a^{-1}} \overline{y(3,2)}$$
$$\xrightarrow{b^{-1}} \overline{y(2,2)} \xrightarrow{b^{-1}} \overline{y(1,2)} \xrightarrow{b^{-1}} \overline{y(0,2)} \xrightarrow{b^{-1}} \overline{y(4,2)} \xrightarrow{a} \overline{xy^2(2,3)}$$
$$\xrightarrow{b} \overline{xy^2(3,3)} \xrightarrow{b} \overline{xy^2(4,3)} \xrightarrow{b} \overline{xy^2(0,3)} \xrightarrow{b} \overline{xy^2(1,3)} \xrightarrow{a^{-1}} \overline{y(3,1)}$$
$$\xrightarrow{b^{-1}} \overline{y(2,1)} \xrightarrow{b^{-1}} \overline{y(1,1)} \xrightarrow{b^{-1}} \overline{y(0,1)} \xrightarrow{b^{-1}} \overline{y(4,1)} \xrightarrow{a^{-1}} \overline{x(3,4)}$$
$$\xrightarrow{b} \overline{x(4,4)} \xrightarrow{b} \overline{x(0,4)} \xrightarrow{b} \overline{x(1,4)} \xrightarrow{b} \overline{x(2,4)} \xrightarrow{a^{-1}} \overline{y^2(3,2)}$$
$$\xrightarrow{b^{-1}} \overline{y^2(2,2)} \xrightarrow{b^{-1}} \overline{y^2(1,2)} \xrightarrow{b^{-1}} \overline{y^2(0,2)} \xrightarrow{b^{-1}} \overline{y^2(4,2)} \xrightarrow{a^{-1}} \overline{xy(2,4)}$$
$$\xrightarrow{a^{-1}} \overline{(3,2)} \xrightarrow{b^{-1}} \overline{(2,2)} \xrightarrow{b^{-1}} \overline{(1,2)} \xrightarrow{b^{-1}} \overline{(0,2)} \xrightarrow{b^{-1}} \overline{(4,2)}$$
$$\xrightarrow{a} \overline{xy(2,3)} \xrightarrow{a} \overline{y^2(3,1)} \xrightarrow{b^{-1}} \overline{y^2(2,1)} \xrightarrow{b^{-1}} \overline{y^2(1,1)} \xrightarrow{b^{-1}} \overline{y^2(0,1)}$$
$$\xrightarrow{b^{-1}} \overline{y^2(4,1)} \xrightarrow{a} \overline{x(1,2)} \xrightarrow{b} \overline{x(2,2)} \xrightarrow{b} \overline{x(3,2)} \xrightarrow{b} \overline{x(4,2)}$$
$$\xrightarrow{b} \overline{x(0,2)} \xrightarrow{a^{-1}} \overline{y^2(3,0)} \xrightarrow{a^{-1}} \overline{xy(3,3)} \xrightarrow{b} \overline{xy(4,3)} \xrightarrow{b} \overline{xy(0,3)}$$
$$\xrightarrow{b} \overline{xy(1,3)} \xrightarrow{a^{-1}} \overline{(3,1)} \xrightarrow{b^{-1}} \overline{(2,1)} \xrightarrow{b^{-1}} \overline{(1,1)} \xrightarrow{b^{-1}} \overline{(0,1)}$$
$$\xrightarrow{b^{-1}} \overline{(4,1)} \xrightarrow{a} \overline{xy(1,2)} \xrightarrow{b} \overline{xy(2,2)} \xrightarrow{b} \overline{xy(3,2)} \xrightarrow{b} \overline{xy(4,2)}$$
$$\xrightarrow{b} \overline{xy(0,2)} \xrightarrow{a^{-1}} \overline{(3,0)} \xrightarrow{b^{-1}} \overline{(2,0)} \xrightarrow{b^{-1}} \overline{(1,0)} \xrightarrow{b^{-1}} \overline{(0,0)}$$

$$S = \{xy, xy(1,0)\} \text{ in } G = (\mathbb{Z}_2 \times \mathbb{Z}_3) \ltimes (\mathbb{Z}_5)^2$$

$$\overline{(0,0)} \xrightarrow{b^{-1}} \overline{xy^2(4,4)} \xrightarrow{b^{-1}} \overline{y(4,3)} \xrightarrow{b^{-1}} \overline{x(0,3)} \xrightarrow{b^{-1}} \overline{y^2(1,4)} \xrightarrow{a^{-1}} \overline{xy(2,1)}$$
$$\xrightarrow{b^{-1}} \overline{(0,1)} \xrightarrow{b^{-1}} \overline{xy^2(3,4)} \xrightarrow{b^{-1}} \overline{y(3,2)} \xrightarrow{b^{-1}} \overline{x(0,2)} \xrightarrow{a^{-1}} \overline{y^2(3,0)}$$
$$\xrightarrow{b} \overline{x(1,2)} \xrightarrow{b} \overline{y(3,1)} \xrightarrow{b} \overline{xy^2(2,3)} \xrightarrow{b} \overline{(4,1)} \xrightarrow{b} \overline{xy(2,2)}$$
$$\xrightarrow{a} \overline{y^2(2,0)} \xrightarrow{b^{-1}} \overline{xy(1,1)} \xrightarrow{b^{-1}} \overline{(4,0)} \xrightarrow{b^{-1}} \overline{xy^2(3,3)} \xrightarrow{b^{-1}} \overline{y(4,2)}$$
$$\xrightarrow{b^{-1}} \overline{x(1,3)} \xrightarrow{a^{-1}} \overline{y^2(3,1)} \xrightarrow{b^{-1}} \overline{xy(1,2)} \xrightarrow{b^{-1}} \overline{(3,0)} \xrightarrow{b^{-1}} \overline{xy^2(2,2)}$$
$$\xrightarrow{b^{-1}} \overline{y(4,1)} \xrightarrow{b^{-1}} \overline{x(2,3)} \xrightarrow{a^{-1}} \overline{y^2(4,2)} \xrightarrow{a^{-1}} \overline{xy(2,4)} \xrightarrow{b^{-1}} \overline{(2,1)}$$
$$\xrightarrow{b^{-1}} \overline{xy^2(0,1)} \xrightarrow{b^{-1}} \overline{y(3,4)} \xrightarrow{b^{-1}} \overline{x(3,2)} \xrightarrow{b^{-1}} \overline{y^2(0,2)} \xrightarrow{a} \overline{x(2,2)}$$
$$\xrightarrow{b} \overline{y(3,0)} \xrightarrow{b} \overline{xy^2(1,2)} \xrightarrow{b} \overline{(3,1)} \xrightarrow{b} \overline{xy(2,3)} \xrightarrow{b} \overline{y^2(4,1)}$$
$$\xrightarrow{a^{-1}} \overline{xy(3,4)} \xrightarrow{b^{-1}} \overline{(3,2)} \xrightarrow{b^{-1}} \overline{xy^2(0,2)} \xrightarrow{b^{-1}} \overline{y(2,4)} \xrightarrow{b^{-1}} \overline{x(2,1)}$$
$$\xrightarrow{b^{-1}} \overline{y^2(0,1)} \xrightarrow{a} \overline{x(1,1)} \xrightarrow{b} \overline{y(2,0)} \xrightarrow{b} \overline{xy^2(1,3)} \xrightarrow{b} \overline{(4,2)}$$
$$\xrightarrow{b} \overline{xy(3,3)} \xrightarrow{b} \overline{y^2(4,0)} \xrightarrow{a^{-1}} \overline{xy(4,4)} \xrightarrow{b^{-1}} \overline{(4,3)} \xrightarrow{b^{-1}} \overline{xy^2(0,3)}$$
$$\xrightarrow{b^{-1}} \overline{y(1,4)} \xrightarrow{b^{-1}} \overline{x(1,0)} \xrightarrow{b^{-1}} \overline{y^2(0,0)} \xrightarrow{a} \overline{x(0,0)} \xrightarrow{b} \overline{y(1,0)}$$
$$\xrightarrow{b} \overline{xy^2(1,4)} \xrightarrow{b} \overline{(0,3)} \xrightarrow{b} \overline{xy(4,3)} \xrightarrow{a} \overline{y^2(3,4)} \xrightarrow{b} \overline{x(0,1)}$$
$$\xrightarrow{b} \overline{y(2,1)} \xrightarrow{b} \overline{xy^2(2,4)} \xrightarrow{b} \overline{(0,2)} \xrightarrow{b} \overline{xy(3,2)} \xrightarrow{a} \overline{y^2(2,4)}$$
$$\xrightarrow{a} \overline{x(4,2)} \xrightarrow{b} \overline{y(3,3)} \xrightarrow{b} \overline{xy^2(4,0)} \xrightarrow{b} \overline{(1,1)} \xrightarrow{b} \overline{xy(2,0)}$$
$$\xrightarrow{b} \overline{y^2(1,3)} \xrightarrow{a^{-1}} \overline{xy(3,1)} \xrightarrow{b^{-1}} \overline{(1,2)} \xrightarrow{b^{-1}} \overline{xy^2(3,0)} \xrightarrow{b^{-1}} \overline{y(2,2)}$$
$$\xrightarrow{b^{-1}} \overline{x(4,1)} \xrightarrow{b^{-1}} \overline{y^2(2,3)} \xrightarrow{a} \overline{x(3,1)} \xrightarrow{b} \overline{y(2,3)} \xrightarrow{b} \overline{xy^2(4,1)}$$
$$\xrightarrow{b} \overline{(2,2)} \xrightarrow{b} \overline{xy(3,0)} \xrightarrow{b} \overline{y^2(1,2)} \xrightarrow{a^{-1}} \overline{xy(4,1)} \xrightarrow{b^{-1}} \overline{(2,3)}$$
$$\xrightarrow{b^{-1}} \overline{xy^2(3,1)} \xrightarrow{b^{-1}} \overline{y(1,2)} \xrightarrow{b^{-1}} \overline{x(3,0)} \xrightarrow{a^{-1}} \overline{y^2(3,3)} \xrightarrow{b^{-1}} \overline{xy(4,2)}$$
$$\xrightarrow{b^{-1}} \overline{(1,3)} \xrightarrow{b^{-1}} \overline{xy^2(2,0)} \xrightarrow{b^{-1}} \overline{y(1,1)} \xrightarrow{b^{-1}} \overline{x(4,0)} \xrightarrow{a^{-1}} \overline{y^2(4,4)}$$
$$\xrightarrow{a^{-1}} \overline{xy(0,4)} \xrightarrow{b^{-1}} \overline{(0,4)} \xrightarrow{b^{-1}} \overline{xy^2(0,4)} \xrightarrow{b^{-1}} \overline{y(0,4)} \xrightarrow{b^{-1}} \overline{x(0,4)}$$
$$\xrightarrow{a^{-1}} \overline{y^2(1,0)} \xrightarrow{b^{-1}} \overline{xy(0,0)} \xrightarrow{b^{-1}} \overline{(4,4)} \xrightarrow{b^{-1}} \overline{xy^2(4,3)} \xrightarrow{b^{-1}} \overline{y(0,3)}$$
$$\xrightarrow{b^{-1}} \overline{x(1,4)} \xrightarrow{a^{-1}} \overline{y^2(2,1)} \xrightarrow{b} \overline{x(2,4)} \xrightarrow{b} \overline{y(0,2)} \xrightarrow{b} \overline{xy^2(3,2)}$$
$$\xrightarrow{b} \overline{(3,4)} \xrightarrow{b} \overline{xy(0,1)} \xrightarrow{a} \overline{y^2(1,1)} \xrightarrow{b^{-1}} \overline{xy(4,0)} \xrightarrow{b^{-1}} \overline{(3,3)}$$
$$\xrightarrow{b^{-1}} \overline{xy^2(4,2)} \xrightarrow{b^{-1}} \overline{y(1,3)} \xrightarrow{b^{-1}} \overline{x(2,0)} \xrightarrow{a^{-1}} \overline{y^2(2,2)} \xrightarrow{a^{-1}} \overline{xy(0,2)}$$
$$\xrightarrow{b^{-1}} \overline{(2,4)} \xrightarrow{b^{-1}} \overline{xy^2(2,1)} \xrightarrow{b^{-1}} \overline{y(0,1)} \xrightarrow{b^{-1}} \overline{x(3,4)} \xrightarrow{b^{-1}} \overline{y^2(3,2)}$$
$$\xrightarrow{a^{-1}} \overline{xy(1,3)} \xrightarrow{b^{-1}} \overline{(2,0)} \xrightarrow{b^{-1}} \overline{xy^2(1,1)} \xrightarrow{b^{-1}} \overline{y(4,0)} \xrightarrow{b^{-1}} \overline{x(3,3)}$$
$$\xrightarrow{a^{-1}} \overline{y^2(0,3)} \xrightarrow{b} \overline{x(4,3)} \xrightarrow{b} \overline{y(4,4)} \xrightarrow{b} \overline{xy^2(0,0)} \xrightarrow{b} \overline{(1,0)}$$
$$\xrightarrow{b} \overline{xy(1,4)} \xrightarrow{a} \overline{y^2(4,3)} \xrightarrow{b^{-1}} \overline{xy(0,3)} \xrightarrow{b^{-1}} \overline{(1,4)} \xrightarrow{b^{-1}} \overline{xy^2(1,0)}$$
$$\xrightarrow{b^{-1}} \overline{y(0,0)} \xrightarrow{b^{-1}} \overline{x(4,4)} \xrightarrow{a^{-1}} \overline{y^2(0,4)} \xrightarrow{a^{-1}} \overline{xy(1,0)} \xrightarrow{b^{-1}} \overline{(0,0)}$$

$$S = \{xy, x(1,0)\} \text{ in } G = (\mathbb{Z}_2 \times \mathbb{Z}_3) \ltimes (\mathbb{Z}_5)^2$$

$$\overline{e} \xrightarrow{a^{-1}} \overline{xy^2(0,0)} \xrightarrow{b} \overline{y^2(1,0)} \xrightarrow{a} \overline{x(0,4)} \xrightarrow{a} \overline{y(4,4)} \xrightarrow{b} \overline{xy(2,1)}$$
$$\xrightarrow{a^{-1}} \overline{(1,2)} \xrightarrow{a^{-1}} \overline{xy^2(4,1)} \xrightarrow{b} \overline{y^2(2,4)} \xrightarrow{a} \overline{x(4,2)} \xrightarrow{a} \overline{y(2,3)}$$
$$\xrightarrow{b} \overline{xy(4,2)} \xrightarrow{a^{-1}} \overline{(2,4)} \xrightarrow{a^{-1}} \overline{xy^2(3,2)} \xrightarrow{a^{-1}} \overline{y(1,3)} \xrightarrow{b} \overline{xy(0,2)}$$
$$\xrightarrow{a^{-1}} \overline{(3,0)} \xrightarrow{a^{-1}} \overline{xy^2(3,3)} \xrightarrow{b} \overline{y^2(3,2)} \xrightarrow{a} \overline{x(2,4)} \xrightarrow{a} \overline{y(4,2)}$$
$$\xrightarrow{b} \overline{xy(2,3)} \xrightarrow{a^{-1}} \overline{(4,2)} \xrightarrow{a^{-1}} \overline{xy^2(2,4)} \xrightarrow{b} \overline{y^2(4,1)} \xrightarrow{a} \overline{x(1,2)}$$
$$\xrightarrow{a} \overline{y(2,1)} \xrightarrow{b} \overline{xy(4,4)} \xrightarrow{a^{-1}} \overline{(0,4)} \xrightarrow{a^{-1}} \overline{xy^2(1,0)} \xrightarrow{a^{-1}} \overline{y(1,1)}$$
$$\xrightarrow{a^{-1}} \overline{x(0,1)} \xrightarrow{a^{-1}} \overline{y^2(4,0)} \xrightarrow{b} \overline{xy^2(2,0)} \xrightarrow{a} \overline{(0,3)} \xrightarrow{a} \overline{xy(3,3)}$$
$$\xrightarrow{b} \overline{y(3,2)} \xrightarrow{a^{-1}} \overline{x(1,3)} \xrightarrow{a^{-1}} \overline{y^2(3,1)} \xrightarrow{b} \overline{xy^2(3,4)} \xrightarrow{a} \overline{(4,1)}$$
$$\xrightarrow{a} \overline{xy(1,2)} \xrightarrow{b} \overline{y(0,3)} \xrightarrow{a^{-1}} \overline{x(2,0)} \xrightarrow{a^{-1}} \overline{y^2(2,2)} \xrightarrow{b} \overline{xy^2(4,3)}$$
$$\xrightarrow{a^{-1}} \overline{y(1,4)} \xrightarrow{b} \overline{xy(0,1)} \xrightarrow{a^{-1}} \overline{(4,0)} \xrightarrow{a^{-1}} \overline{xy^2(4,4)} \xrightarrow{b} \overline{y^2(2,1)}$$
$$\xrightarrow{a} \overline{x(1,4)} \xrightarrow{a} \overline{y(4,3)} \xrightarrow{b} \overline{xy(2,2)} \xrightarrow{a^{-1}} \overline{(0,2)} \xrightarrow{a^{-1}} \overline{xy^2(3,0)}$$
$$\xrightarrow{b} \overline{y^2(3,0)} \xrightarrow{a} \overline{x(0,2)} \xrightarrow{a} \overline{y(2,2)} \xrightarrow{b} \overline{xy(4,3)} \xrightarrow{a^{-1}} \overline{(1,4)}$$
$$\xrightarrow{a^{-1}} \overline{xy^2(2,1)} \xrightarrow{a^{-1}} \overline{y(1,2)} \xrightarrow{a^{-1}} \overline{x(4,1)} \xrightarrow{a^{-1}} \overline{y^2(3,4)} \xrightarrow{b} \overline{xy^2(3,1)}$$
$$\xrightarrow{a} \overline{(1,3)} \xrightarrow{a} \overline{xy(3,2)} \xrightarrow{b} \overline{y(3,3)} \xrightarrow{a^{-1}} \overline{x(0,3)} \xrightarrow{a^{-1}} \overline{y^2(2,0)}$$
$$\xrightarrow{b} \overline{xy^2(4,0)} \xrightarrow{a} \overline{(0,1)} \xrightarrow{a} \overline{xy(1,1)} \xrightarrow{b} \overline{y(0,4)} \xrightarrow{a^{-1}} \overline{x(1,0)}$$
$$\xrightarrow{a^{-1}} \overline{y^2(1,1)} \xrightarrow{b} \overline{xy^2(0,4)} \xrightarrow{a^{-1}} \overline{y(1,0)} \xrightarrow{a^{-1}} \overline{x(1,1)} \xrightarrow{a^{-1}} \overline{y^2(0,1)}$$
$$\xrightarrow{b} \overline{xy^2(1,4)} \xrightarrow{a} \overline{(4,3)} \xrightarrow{a} \overline{xy(3,4)} \xrightarrow{b} \overline{y(3,1)} \xrightarrow{a^{-1}} \overline{x(2,3)}$$
$$\xrightarrow{a^{-1}} \overline{y^2(4,2)} \xrightarrow{b} \overline{xy^2(2,3)} \xrightarrow{a} \overline{(3,1)} \xrightarrow{a} \overline{xy(1,3)} \xrightarrow{b} \overline{y(0,2)}$$
$$\xrightarrow{a^{-1}} \overline{x(3,0)} \xrightarrow{a^{-1}} \overline{y^2(3,3)} \xrightarrow{a^{-1}} \overline{xy(0,3)} \xrightarrow{a^{-1}} \overline{(2,0)} \xrightarrow{a^{-1}} \overline{xy^2(2,2)}$$
$$\xrightarrow{b} \overline{y^2(4,3)} \xrightarrow{a} \overline{x(3,4)} \xrightarrow{a} \overline{y(4,1)} \xrightarrow{b} \overline{xy(2,4)} \xrightarrow{a^{-1}} \overline{(3,2)}$$
$$\xrightarrow{a^{-1}} \overline{xy^2(1,3)} \xrightarrow{b} \overline{y^2(0,2)} \xrightarrow{a} \overline{x(2,2)} \xrightarrow{a} \overline{y(2,0)} \xrightarrow{b} \overline{xy(4,0)}$$
$$\xrightarrow{a^{-1}} \overline{(4,4)} \xrightarrow{b} \overline{x(2,1)} \xrightarrow{a^{-1}} \overline{y^2(1,2)} \xrightarrow{b} \overline{xy^2(0,3)} \xrightarrow{a} \overline{(3,3)}$$
$$\xrightarrow{a} \overline{xy(3,0)} \xrightarrow{b} \overline{y(3,0)} \xrightarrow{a^{-1}} \overline{x(3,3)} \xrightarrow{a^{-1}} \overline{y^2(0,3)} \xrightarrow{b} \overline{xy^2(1,2)}$$
$$\xrightarrow{a} \overline{(2,1)} \xrightarrow{a} \overline{xy(1,4)} \xrightarrow{b} \overline{y(0,1)} \xrightarrow{a^{-1}} \overline{x(4,0)} \xrightarrow{a^{-1}} \overline{y^2(4,4)}$$
$$\xrightarrow{a^{-1}} \overline{xy(0,4)} \xrightarrow{a^{-1}} \overline{(1,0)} \xrightarrow{a^{-1}} \overline{xy^2(1,1)} \xrightarrow{b} \overline{y^2(0,4)} \xrightarrow{a} \overline{x(4,4)}$$
$$\xrightarrow{a} \overline{y(4,0)} \xrightarrow{b} \overline{xy(2,0)} \xrightarrow{a^{-1}} \overline{(2,2)} \xrightarrow{a^{-1}} \overline{xy^2(0,2)} \xrightarrow{b} \overline{y^2(1,3)}$$
$$\xrightarrow{a} \overline{x(3,2)} \xrightarrow{a} \overline{y(2,4)} \xrightarrow{b} \overline{xy(4,1)} \xrightarrow{a^{-1}} \overline{(3,4)} \xrightarrow{b} \overline{x(3,1)}$$
$$\xrightarrow{a^{-1}} \overline{y^2(2,3)} \xrightarrow{b} \overline{xy^2(4,2)} \xrightarrow{a} \overline{(2,3)} \xrightarrow{a} \overline{xy(3,1)} \xrightarrow{b} \overline{y(3,4)}$$
$$\xrightarrow{a^{-1}} \overline{x(4,3)} \xrightarrow{a^{-1}} \overline{y^2(1,4)} \xrightarrow{b} \overline{xy^2(0,1)} \xrightarrow{a} \overline{(1,1)} \xrightarrow{a} \overline{xy(1,0)}$$
$$\xrightarrow{b} \overline{y(0,0)} \xrightarrow{a^{-1}} \overline{x(0,0)} \xrightarrow{a^{-1}} \overline{y^2(0,0)} \xrightarrow{a^{-1}} \overline{xy(0,0)} \xrightarrow{a^{-1}} \overline{(0,0)}$$

$$S = \{xy, y(1,0)\} \text{ in } G = (\mathbb{Z}_2 \times \mathbb{Z}_3) \ltimes (\mathbb{Z}_5)^2$$

$$\overline{e} \xrightarrow{a^{-1}} \overline{xy^2(0,0)} \xrightarrow{a^{-1}} \overline{y(0,0)} \xrightarrow{a^{-1}} \overline{x(0,0)} \xrightarrow{a^{-1}} \overline{y^2(0,0)} \xrightarrow{b^{-1}} \overline{y(1,1)}$$
$$\xrightarrow{a} \overline{xy^2(1,0)} \xrightarrow{a} \overline{(0,4)} \xrightarrow{a} \overline{xy(4,4)} \xrightarrow{a} \overline{y^2(4,0)} \xrightarrow{a} \overline{x(0,1)}$$
$$\xrightarrow{b} \overline{xy(0,4)} \xrightarrow{a^{-1}} \overline{(1,0)} \xrightarrow{a^{-1}} \overline{xy^2(1,1)} \xrightarrow{a^{-1}} \overline{y(0,1)} \xrightarrow{a^{-1}} \overline{x(4,0)}$$
$$\xrightarrow{a^{-1}} \overline{y^2(4,4)} \xrightarrow{b^{-1}} \overline{y(1,2)} \xrightarrow{a} \overline{xy^2(2,1)} \xrightarrow{a} \overline{(1,4)} \xrightarrow{a} \overline{xy(4,3)}$$
$$\xrightarrow{a} \overline{y^2(3,4)} \xrightarrow{a} \overline{x(4,1)} \xrightarrow{b} \overline{xy(0,3)} \xrightarrow{a^{-1}} \overline{(2,0)} \xrightarrow{a^{-1}} \overline{xy^2(2,2)}$$
$$\xrightarrow{a^{-1}} \overline{y(0,2)} \xrightarrow{a^{-1}} \overline{x(3,0)} \xrightarrow{a^{-1}} \overline{y^2(3,3)} \xrightarrow{b^{-1}} \overline{y(1,3)} \xrightarrow{a} \overline{xy^2(3,2)}$$
$$\xrightarrow{a} \overline{(2,4)} \xrightarrow{a} \overline{xy(4,2)} \xrightarrow{b} \overline{xy^2(4,2)} \xrightarrow{a} \overline{(2,3)} \xrightarrow{a} \overline{xy(3,1)}$$
$$\xrightarrow{b^{-1}} \overline{x(4,3)} \xrightarrow{a^{-1}} \overline{y^2(1,4)} \xrightarrow{b^{-1}} \overline{y(4,0)} \xrightarrow{a^{-1}} \overline{x(4,4)} \xrightarrow{a^{-1}} \overline{y^2(0,4)}$$
$$\xrightarrow{a^{-1}} \overline{xy(1,0)} \xrightarrow{a^{-1}} \overline{(1,1)} \xrightarrow{a^{-1}} \overline{xy^2(0,1)} \xrightarrow{b^{-1}} \overline{xy(2,1)} \xrightarrow{a^{-1}} \overline{(1,2)}$$
$$\xrightarrow{a^{-1}} \overline{xy^2(4,1)} \xrightarrow{a^{-1}} \overline{y(3,4)} \xrightarrow{b} \overline{y^2(2,4)} \xrightarrow{a} \overline{x(4,2)} \xrightarrow{a} \overline{y(2,3)}$$
$$\xrightarrow{a} \overline{xy^2(3,1)} \xrightarrow{a} \overline{(1,3)} \xrightarrow{a} \overline{xy(3,2)} \xrightarrow{b^{-1}} \overline{x(0,3)} \xrightarrow{a^{-1}} \overline{y^2(2,0)}$$
$$\xrightarrow{b^{-1}} \overline{y(4,4)} \xrightarrow{a^{-1}} \overline{x(0,4)} \xrightarrow{a^{-1}} \overline{y^2(1,0)} \xrightarrow{a^{-1}} \overline{xy(1,1)} \xrightarrow{a^{-1}} \overline{(0,1)}$$
$$\xrightarrow{a^{-1}} \overline{xy^2(4,0)} \xrightarrow{b^{-1}} \overline{xy(2,2)} \xrightarrow{a^{-1}} \overline{(0,2)} \xrightarrow{a^{-1}} \overline{xy^2(3,0)} \xrightarrow{a^{-1}} \overline{y(3,3)}$$
$$\xrightarrow{b} \overline{y^2(3,0)} \xrightarrow{a} \overline{x(0,2)} \xrightarrow{a} \overline{y(2,2)} \xrightarrow{a} \overline{xy^2(2,0)} \xrightarrow{a} \overline{(0,3)}$$
$$\xrightarrow{a} \overline{xy(3,3)} \xrightarrow{b^{-1}} \overline{x(1,3)} \xrightarrow{a^{-1}} \overline{y^2(3,1)} \xrightarrow{b^{-1}} \overline{y(4,3)} \xrightarrow{a^{-1}} \overline{x(1,4)}$$
$$\xrightarrow{a^{-1}} \overline{y^2(2,1)} \xrightarrow{a^{-1}} \overline{xy(1,2)} \xrightarrow{a^{-1}} \overline{(4,1)} \xrightarrow{a^{-1}} \overline{xy^2(3,4)} \xrightarrow{b^{-1}} \overline{xy(2,3)}$$
$$\xrightarrow{a^{-1}} \overline{(4,2)} \xrightarrow{a^{-1}} \overline{xy^2(2,4)} \xrightarrow{a^{-1}} \overline{y(3,2)} \xrightarrow{b} \overline{y^2(4,1)} \xrightarrow{a} \overline{x(1,2)}$$
$$\xrightarrow{a} \overline{y(2,1)} \xrightarrow{a} \overline{xy^2(1,4)} \xrightarrow{a} \overline{(4,3)} \xrightarrow{a} \overline{xy(3,4)} \xrightarrow{b^{-1}} \overline{x(2,3)}$$
$$\xrightarrow{a^{-1}} \overline{y^2(4,2)} \xrightarrow{b^{-1}} \overline{y(4,2)} \xrightarrow{a^{-1}} \overline{x(2,4)} \xrightarrow{a^{-1}} \overline{y^2(3,2)} \xrightarrow{a^{-1}} \overline{xy(1,3)}$$
$$\xrightarrow{a^{-1}} \overline{(3,1)} \xrightarrow{a^{-1}} \overline{xy^2(2,3)} \xrightarrow{b^{-1}} \overline{xy(2,4)} \xrightarrow{a^{-1}} \overline{(3,2)} \xrightarrow{a^{-1}} \overline{xy^2(1,3)}$$
$$\xrightarrow{a^{-1}} \overline{y(3,1)} \xrightarrow{b} \overline{y^2(0,2)} \xrightarrow{a} \overline{x(2,2)} \xrightarrow{a} \overline{y(2,0)} \xrightarrow{a} \overline{xy^2(0,3)}$$
$$\xrightarrow{a} \overline{(3,3)} \xrightarrow{a} \overline{xy(3,0)} \xrightarrow{b^{-1}} \overline{x(3,3)} \xrightarrow{a^{-1}} \overline{y^2(0,3)} \xrightarrow{b^{-1}} \overline{y(4,1)}$$
$$\xrightarrow{a^{-1}} \overline{x(3,4)} \xrightarrow{a^{-1}} \overline{y^2(4,3)} \xrightarrow{a^{-1}} \overline{xy(1,4)} \xrightarrow{a^{-1}} \overline{(2,1)} \xrightarrow{a^{-1}} \overline{xy^2(1,2)}$$
$$\xrightarrow{b^{-1}} \overline{xy(2,0)} \xrightarrow{a^{-1}} \overline{(2,2)} \xrightarrow{a^{-1}} \overline{xy^2(0,2)} \xrightarrow{a^{-1}} \overline{y(3,0)} \xrightarrow{b} \overline{y^2(1,3)}$$
$$\xrightarrow{a} \overline{x(3,2)} \xrightarrow{a} \overline{y(2,4)} \xrightarrow{b} \overline{y^2(2,3)} \xrightarrow{a} \overline{x(3,1)} \xrightarrow{b} \overline{xy(0,2)}$$
$$\xrightarrow{a^{-1}} \overline{(3,0)} \xrightarrow{a^{-1}} \overline{xy^2(3,3)} \xrightarrow{a^{-1}} \overline{y(0,3)} \xrightarrow{a^{-1}} \overline{x(2,0)} \xrightarrow{a^{-1}} \overline{y^2(2,2)}$$
$$\xrightarrow{b^{-1}} \overline{y(1,4)} \xrightarrow{a} \overline{xy^2(4,3)} \xrightarrow{a} \overline{(3,4)} \xrightarrow{a} \overline{xy(4,1)} \xrightarrow{a} \overline{y^2(1,2)}$$
$$\xrightarrow{a} \overline{x(2,1)} \xrightarrow{b} \overline{xy(0,1)} \xrightarrow{a^{-1}} \overline{(4,0)} \xrightarrow{a^{-1}} \overline{xy^2(4,4)} \xrightarrow{a^{-1}} \overline{y(0,4)}$$
$$\xrightarrow{a^{-1}} \overline{x(1,0)} \xrightarrow{a^{-1}} \overline{y^2(1,1)} \xrightarrow{b^{-1}} \overline{y(1,0)} \xrightarrow{a} \overline{xy^2(0,4)} \xrightarrow{a} \overline{(4,4)}$$
$$\xrightarrow{a} \overline{xy(4,0)} \xrightarrow{a} \overline{y^2(0,1)} \xrightarrow{a} \overline{x(1,1)} \xrightarrow{b} \overline{xy(0,0)} \xrightarrow{a^{-1}} \overline{(0,0)}$$

$$S = \{x, y(1,0)\} \text{ in } G = (\mathbb{Z}_2 \times \mathbb{Z}_3) \ltimes (\mathbb{Z}_5)^2$$

$$\overline{(0,0)} \xrightarrow{b} \overline{y(1,0)} \xrightarrow{b} \overline{y^2(1,1)} \xrightarrow{a} \overline{xy^2(4,4)} \xrightarrow{b^{-1}} \overline{xy(1,2)} \xrightarrow{b^{-1}} \overline{x(2,0)}$$
$$\xrightarrow{a} \overline{(3,0)} \xrightarrow{b} \overline{y(1,3)} \xrightarrow{b} \overline{y^2(3,3)} \xrightarrow{a} \overline{xy^2(2,2)} \xrightarrow{b^{-1}} \overline{xy(1,4)}$$
$$\xrightarrow{b^{-1}} \overline{x(4,0)} \xrightarrow{a} \overline{(1,0)} \xrightarrow{b} \overline{y(1,1)} \xrightarrow{b} \overline{y^2(0,0)} \xrightarrow{a} \overline{xy^2(0,0)}$$
$$\xrightarrow{b^{-1}} \overline{xy(1,1)} \xrightarrow{b^{-1}} \overline{x(1,0)} \xrightarrow{a} \overline{(4,0)} \xrightarrow{b^{-1}} \overline{y^2(2,2)} \xrightarrow{b^{-1}} \overline{y(1,4)}$$
$$\xrightarrow{a} \overline{xy(4,1)} \xrightarrow{b} \overline{xy^2(0,3)} \xrightarrow{b} \overline{x(3,2)} \xrightarrow{a} \overline{(2,3)} \xrightarrow{b} \overline{y(3,4)}$$
$$\xrightarrow{b} \overline{y^2(2,4)} \xrightarrow{a} \overline{xy^2(3,1)} \xrightarrow{b^{-1}} \overline{xy(4,3)} \xrightarrow{b^{-1}} \overline{x(0,2)} \xrightarrow{a} \overline{(0,3)}$$
$$\xrightarrow{b} \overline{y(3,2)} \xrightarrow{b} \overline{y^2(4,1)} \xrightarrow{a} \overline{xy^2(1,4)} \xrightarrow{b^{-1}} \overline{xy(4,0)} \xrightarrow{b^{-1}} \overline{x(2,2)}$$
$$\xrightarrow{a} \overline{(3,3)} \xrightarrow{b} \overline{y(3,0)} \xrightarrow{b} \overline{y^2(1,3)} \xrightarrow{a} \overline{xy^2(4,2)} \xrightarrow{b^{-1}} \overline{xy(4,2)}$$
$$\xrightarrow{b^{-1}} \overline{x(4,2)} \xrightarrow{a} \overline{(1,3)} \xrightarrow{b} \overline{y(3,3)} \xrightarrow{b} \overline{y^2(3,0)} \xrightarrow{a} \overline{xy^2(2,0)}$$
$$\xrightarrow{b^{-1}} \overline{xy(4,4)} \xrightarrow{b^{-1}} \overline{x(1,2)} \xrightarrow{a} \overline{(4,3)} \xrightarrow{b^{-1}} \overline{y^2(0,2)} \xrightarrow{b^{-1}} \overline{y(3,1)}$$
$$\xrightarrow{a} \overline{xy(2,4)} \xrightarrow{b} \overline{xy^2(2,3)} \xrightarrow{b} \overline{x(3,4)} \xrightarrow{a} \overline{(2,1)} \xrightarrow{b} \overline{y(0,1)}$$
$$\xrightarrow{b} \overline{y^2(0,4)} \xrightarrow{a} \overline{xy^2(0,1)} \xrightarrow{b^{-1}} \overline{xy(2,1)} \xrightarrow{b^{-1}} \overline{x(0,4)} \xrightarrow{a} \overline{(0,1)}$$
$$\xrightarrow{b} \overline{y(0,4)} \xrightarrow{b} \overline{y^2(2,1)} \xrightarrow{a} \overline{xy^2(3,4)} \xrightarrow{b^{-1}} \overline{xy(2,3)} \xrightarrow{b^{-1}} \overline{x(2,4)}$$
$$\xrightarrow{a} \overline{(3,1)} \xrightarrow{b} \overline{y(0,2)} \xrightarrow{b} \overline{y^2(4,3)} \xrightarrow{a} \overline{xy^2(1,2)} \xrightarrow{b^{-1}} \overline{xy(2,0)}$$
$$\xrightarrow{b^{-1}} \overline{x(4,4)} \xrightarrow{a} \overline{(1,1)} \xrightarrow{b} \overline{y(0,0)} \xrightarrow{b} \overline{y^2(1,0)} \xrightarrow{a} \overline{xy^2(4,0)}$$
$$\xrightarrow{b^{-1}} \overline{xy(2,2)} \xrightarrow{b^{-1}} \overline{x(1,4)} \xrightarrow{a} \overline{(4,1)} \xrightarrow{b^{-1}} \overline{y^2(3,2)} \xrightarrow{b^{-1}} \overline{y(0,3)}$$
$$\xrightarrow{a} \overline{xy(0,2)} \xrightarrow{b} \overline{xy^2(4,3)} \xrightarrow{b} \overline{x(3,1)} \xrightarrow{a} \overline{(2,4)} \xrightarrow{b} \overline{y(2,3)}$$
$$\xrightarrow{b} \overline{y^2(3,4)} \xrightarrow{a} \overline{xy^2(2,1)} \xrightarrow{b^{-1}} \overline{xy(0,4)} \xrightarrow{b^{-1}} \overline{x(0,1)} \xrightarrow{a} \overline{(0,4)}$$
$$\xrightarrow{b} \overline{y(2,1)} \xrightarrow{b} \overline{y^2(0,1)} \xrightarrow{a} \overline{xy^2(0,4)} \xrightarrow{b^{-1}} \overline{xy(0,1)} \xrightarrow{b^{-1}} \overline{x(2,1)}$$
$$\xrightarrow{a} \overline{(3,4)} \xrightarrow{b} \overline{y(2,4)} \xrightarrow{b} \overline{y^2(2,3)} \xrightarrow{a} \overline{xy^2(3,2)} \xrightarrow{b^{-1}} \overline{xy(0,3)}$$
$$\xrightarrow{b^{-1}} \overline{x(4,1)} \xrightarrow{a} \overline{(1,4)} \xrightarrow{b} \overline{y(2,2)} \xrightarrow{b} \overline{y^2(4,0)} \xrightarrow{a} \overline{xy^2(1,0)}$$
$$\xrightarrow{b^{-1}} \overline{xy(0,0)} \xrightarrow{b^{-1}} \overline{x(1,1)} \xrightarrow{a} \overline{(4,4)} \xrightarrow{b^{-1}} \overline{y^2(1,2)} \xrightarrow{b^{-1}} \overline{y(2,0)}$$
$$\xrightarrow{a} \overline{xy(3,0)} \xrightarrow{b} \overline{xy^2(1,3)} \xrightarrow{b} \overline{x(3,3)} \xrightarrow{a} \overline{(2,2)} \xrightarrow{b} \overline{y(4,0)}$$
$$\xrightarrow{b} \overline{y^2(1,4)} \xrightarrow{a} \overline{xy^2(4,1)} \xrightarrow{b^{-1}} \overline{xy(3,2)} \xrightarrow{b^{-1}} \overline{x(0,3)} \xrightarrow{a} \overline{(0,2)}$$
$$\xrightarrow{b} \overline{y(4,3)} \xrightarrow{b} \overline{y^2(3,1)} \xrightarrow{a} \overline{xy^2(2,4)} \xrightarrow{b^{-1}} \overline{xy(3,4)} \xrightarrow{b^{-1}} \overline{x(2,3)}$$
$$\xrightarrow{a} \overline{(3,2)} \xrightarrow{b} \overline{y(4,1)} \xrightarrow{b} \overline{y^2(0,3)} \xrightarrow{a} \overline{xy^2(0,2)} \xrightarrow{b^{-1}} \overline{xy(3,1)}$$
$$\xrightarrow{b^{-1}} \overline{x(4,3)} \xrightarrow{a} \overline{(1,2)} \xrightarrow{b} \overline{y(4,4)} \xrightarrow{b} \overline{y^2(2,0)} \xrightarrow{a} \overline{xy^2(3,0)}$$
$$\xrightarrow{b^{-1}} \overline{xy(3,3)} \xrightarrow{b^{-1}} \overline{x(1,3)} \xrightarrow{a} \overline{(4,2)} \xrightarrow{b^{-1}} \overline{y^2(4,2)} \xrightarrow{b^{-1}} \overline{y(4,2)}$$
$$\xrightarrow{a} \overline{xy(1,3)} \xrightarrow{b} \overline{xy^2(3,3)} \xrightarrow{b} \overline{x(3,0)} \xrightarrow{a} \overline{(2,0)} \xrightarrow{b} \overline{y(1,2)}$$
$$\xrightarrow{b} \overline{y^2(4,4)} \xrightarrow{a} \overline{xy^2(1,1)} \xrightarrow{b^{-1}} \overline{xy(1,0)} \xrightarrow{b^{-1}} \overline{x(0,0)} \xrightarrow{a} \overline{(0,0)}$$

$S = \{x, y, (1,0)\}$ in $G = (\mathbb{Z}_2 \times \mathbb{Z}_3) \ltimes (\mathbb{Z}_5)^2$

$$\overline{(0,0)} \xrightarrow{b} \overline{y(0,0)} \xrightarrow{a} \overline{xy(0,0)} \xrightarrow{c^{-1}} \overline{xy(4,0)} \xrightarrow{a} \overline{y(1,0)} \xrightarrow{b^{-1}} \overline{(4,4)}$$
$$\xrightarrow{a} \overline{x(1,1)} \xrightarrow{b^{-1}} \overline{xy^2(0,4)} \xrightarrow{a} \overline{y^2(0,1)} \xrightarrow{c} \overline{y^2(1,1)} \xrightarrow{a} \overline{xy^2(4,4)}$$
$$\xrightarrow{b} \overline{x(1,0)} \xrightarrow{a} \overline{(4,0)} \xrightarrow{b} \overline{y(0,4)} \xrightarrow{a} \overline{xy(0,1)} \xrightarrow{c^{-1}} \overline{xy(4,1)}$$
$$\xrightarrow{a} \overline{y(1,4)} \xrightarrow{b^{-1}} \overline{(3,4)} \xrightarrow{a} \overline{x(2,1)} \xrightarrow{b^{-1}} \overline{xy^2(4,3)} \xrightarrow{a} \overline{y^2(1,2)}$$
$$\xrightarrow{c^{-1}} \overline{y^2(0,2)} \xrightarrow{a} \overline{xy^2(0,3)} \xrightarrow{b^{-1}} \overline{xy(3,0)} \xrightarrow{a} \overline{y(2,0)} \xrightarrow{b^{-1}} \overline{(3,3)}$$
$$\xrightarrow{a} \overline{x(2,2)} \xrightarrow{c^{-1}} \overline{x(1,2)} \xrightarrow{a} \overline{(4,3)} \xrightarrow{b} \overline{y(2,1)} \xrightarrow{a} \overline{xy(3,4)}$$
$$\xrightarrow{c} \overline{xy(4,4)} \xrightarrow{a} \overline{y(1,1)} \xrightarrow{b^{-1}} \overline{(0,4)} \xrightarrow{a} \overline{x(0,1)} \xrightarrow{b^{-1}} \overline{xy^2(1,0)}$$
$$\xrightarrow{a} \overline{y^2(4,0)} \xrightarrow{c^{-1}} \overline{y^2(3,0)} \xrightarrow{c^{-1}} \overline{y^2(2,0)} \xrightarrow{a} \overline{xy^2(3,0)} \xrightarrow{c^{-1}} \overline{xy^2(2,0)}$$
$$\xrightarrow{b} \overline{x(0,2)} \xrightarrow{a} \overline{(0,3)} \xrightarrow{b} \overline{y(2,2)} \xrightarrow{a} \overline{xy(3,3)} \xrightarrow{c} \overline{xy(4,3)}$$
$$\xrightarrow{a} \overline{y(1,2)} \xrightarrow{b^{-1}} \overline{(1,4)} \xrightarrow{a} \overline{x(4,1)} \xrightarrow{b^{-1}} \overline{xy^2(2,1)} \xrightarrow{c} \overline{xy^2(3,1)}$$
$$\xrightarrow{a} \overline{y^2(2,4)} \xrightarrow{c} \overline{y^2(3,4)} \xrightarrow{c} \overline{y^2(4,4)} \xrightarrow{a} \overline{xy^2(1,1)} \xrightarrow{b^{-1}} \overline{xy(0,4)}$$
$$\xrightarrow{a} \overline{y(0,1)} \xrightarrow{b^{-1}} \overline{(1,0)} \xrightarrow{a} \overline{x(4,0)} \xrightarrow{c^{-1}} \overline{x(3,0)} \xrightarrow{a} \overline{(2,0)}$$
$$\xrightarrow{b} \overline{y(0,2)} \xrightarrow{a} \overline{xy(0,3)} \xrightarrow{b} \overline{xy^2(2,2)} \xrightarrow{c^{-1}} \overline{xy^2(1,2)} \xrightarrow{a} \overline{y^2(4,3)}$$
$$\xrightarrow{c^{-1}} \overline{y^2(3,3)} \xrightarrow{c^{-1}} \overline{y^2(2,3)} \xrightarrow{a} \overline{xy^2(3,2)} \xrightarrow{b} \overline{x(3,1)} \xrightarrow{a} \overline{(2,4)}$$
$$\xrightarrow{b} \overline{y(1,3)} \xrightarrow{a} \overline{xy(4,2)} \xrightarrow{c} \overline{xy(0,2)} \xrightarrow{a} \overline{y(0,3)} \xrightarrow{b^{-1}} \overline{(3,0)}$$
$$\xrightarrow{a} \overline{x(2,0)} \xrightarrow{b^{-1}} \overline{xy^2(3,3)} \xrightarrow{a} \overline{y^2(2,2)} \xrightarrow{c} \overline{y^2(3,2)} \xrightarrow{c} \overline{y^2(4,2)}$$
$$\xrightarrow{a} \overline{xy^2(1,3)} \xrightarrow{c} \overline{xy^2(2,3)} \xrightarrow{b^{-1}} \overline{xy(1,3)} \xrightarrow{a} \overline{y(4,2)} \xrightarrow{b^{-1}} \overline{(3,1)}$$
$$\xrightarrow{a} \overline{x(2,4)} \xrightarrow{c^{-1}} \overline{x(1,4)} \xrightarrow{a} \overline{(4,1)} \xrightarrow{b} \overline{y(4,3)} \xrightarrow{a} \overline{xy(1,2)}$$
$$\xrightarrow{b} \overline{xy^2(3,4)} \xrightarrow{a} \overline{y^2(2,1)} \xrightarrow{c} \overline{y^2(3,1)} \xrightarrow{c} \overline{y^2(4,1)} \xrightarrow{a} \overline{xy^2(1,4)}$$
$$\xrightarrow{c} \overline{xy^2(2,4)} \xrightarrow{b^{-1}} \overline{xy(2,3)} \xrightarrow{a} \overline{y(3,2)} \xrightarrow{b^{-1}} \overline{(4,2)} \xrightarrow{a} \overline{x(1,3)}$$
$$\xrightarrow{c^{-1}} \overline{x(0,3)} \xrightarrow{a} \overline{(0,2)} \xrightarrow{b} \overline{y(3,3)} \xrightarrow{a} \overline{xy(2,2)} \xrightarrow{c} \overline{xy(3,2)}$$
$$\xrightarrow{a} \overline{y(2,3)} \xrightarrow{b^{-1}} \overline{(1,3)} \xrightarrow{a} \overline{x(4,2)} \xrightarrow{c^{-1}} \overline{x(3,2)} \xrightarrow{a} \overline{(2,3)}$$
$$\xrightarrow{b} \overline{y(2,4)} \xrightarrow{a} \overline{xy(3,1)} \xrightarrow{b} \overline{xy^2(4,2)} \xrightarrow{a} \overline{y^2(1,3)} \xrightarrow{c^{-1}} \overline{y^2(0,3)}$$
$$\xrightarrow{a} \overline{xy^2(0,2)} \xrightarrow{b^{-1}} \overline{xy(2,0)} \xrightarrow{a} \overline{y(3,0)} \xrightarrow{b^{-1}} \overline{(2,2)} \xrightarrow{a} \overline{x(3,3)}$$
$$\xrightarrow{c^{-1}} \overline{x(2,3)} \xrightarrow{a} \overline{(3,2)} \xrightarrow{b} \overline{y(3,1)} \xrightarrow{a} \overline{xy(2,4)} \xrightarrow{c^{-1}} \overline{xy(1,4)}$$
$$\xrightarrow{a} \overline{y(4,1)} \xrightarrow{b^{-1}} \overline{(2,1)} \xrightarrow{a} \overline{x(3,4)} \xrightarrow{c} \overline{x(4,4)} \xrightarrow{a} \overline{(1,1)}$$
$$\xrightarrow{b} \overline{y(4,0)} \xrightarrow{a} \overline{xy(1,0)} \xrightarrow{b} \overline{xy^2(0,1)} \xrightarrow{a} \overline{y^2(0,4)} \xrightarrow{c} \overline{y^2(1,4)}$$
$$\xrightarrow{a} \overline{xy^2(4,1)} \xrightarrow{b} \overline{x(4,3)} \xrightarrow{a} \overline{(1,2)} \xrightarrow{b} \overline{y(3,4)} \xrightarrow{a} \overline{xy(2,1)}$$
$$\xrightarrow{c^{-1}} \overline{xy(1,1)} \xrightarrow{a} \overline{y(4,4)} \xrightarrow{b^{-1}} \overline{(0,1)} \xrightarrow{a} \overline{x(0,4)} \xrightarrow{b^{-1}} \overline{xy^2(4,0)}$$
$$\xrightarrow{a} \overline{y^2(1,0)} \xrightarrow{c^{-1}} \overline{y^2(0,0)} \xrightarrow{a} \overline{xy^2(0,0)} \xrightarrow{b} \overline{x(0,0)} \xrightarrow{a} \overline{(0,0)}$$

$f$ inverts $t$, $t$ is nontrivial on $P$, and $S = \{f(1,0), t\}$

$$
\begin{array}{ccccccccccc}
\overline{(0,0)} & \xrightarrow{a^{-1}} & \overline{f(4,0)} & \xrightarrow{a^{-1}} & \overline{(3,0)} & \xrightarrow{a^{-1}} & \overline{f(2,0)} & \xrightarrow{a^{-1}} & \overline{(1,0)} & \xrightarrow{a^{-1}} & \overline{f(0,0)} \\
& \xrightarrow{a^{-1}} & \overline{(4,0)} & \xrightarrow{b} & \overline{t(3,4)} & \xrightarrow{b} & \overline{t^2(3,1)} & \xrightarrow{a^{-1}} & \overline{ft(2,4)} & \xrightarrow{b} & \overline{ft^2(1,0)} \\
& \xrightarrow{a^{-1}} & \overline{t(0,0)} & \xrightarrow{a^{-1}} & \overline{ft^2(4,0)} & \xrightarrow{b} & \overline{f(3,4)} & \xrightarrow{a^{-1}} & \overline{(2,1)} & \xrightarrow{a^{-1}} & \overline{f(1,4)} \\
& \xrightarrow{a^{-1}} & \overline{(0,1)} & \xrightarrow{a^{-1}} & \overline{f(4,4)} & \xrightarrow{a^{-1}} & \overline{(3,1)} & \xrightarrow{a^{-1}} & \overline{f(2,4)} & \xrightarrow{a^{-1}} & \overline{(1,1)} \\
& \xrightarrow{a^{-1}} & \overline{f(0,4)} & \xrightarrow{a^{-1}} & \overline{(4,1)} & \xrightarrow{b} & \overline{t(1,1)} & \xrightarrow{a} & \overline{ft^2(2,4)} & \xrightarrow{a} & \overline{t(3,1)} \\
& \xrightarrow{a} & \overline{ft^2(4,4)} & \xrightarrow{a} & \overline{t(0,1)} & \xrightarrow{a} & \overline{ft^2(1,4)} & \xrightarrow{b^{-1}} & \overline{ft(0,2)} & \xrightarrow{a^{-1}} & \overline{t^2(4,3)} \\
& \xrightarrow{b^{-1}} & \overline{t(4,2)} & \xrightarrow{a^{-1}} & \overline{ft^2(3,3)} & \xrightarrow{a^{-1}} & \overline{t(2,2)} & \xrightarrow{a^{-1}} & \overline{ft^2(1,3)} & \xrightarrow{a^{-1}} & \overline{t(0,2)} \\
& \xrightarrow{b^{-1}} & \overline{(4,4)} & \xrightarrow{a} & \overline{f(0,1)} & \xrightarrow{a} & \overline{(1,4)} & \xrightarrow{a} & \overline{f(2,1)} & \xrightarrow{a} & \overline{(3,4)} \\
& \xrightarrow{a} & \overline{f(4,1)} & \xrightarrow{a} & \overline{(0,4)} & \xrightarrow{a} & \overline{f(1,1)} & \xrightarrow{a} & \overline{(2,4)} & \xrightarrow{a} & \overline{f(3,1)} \\
& \xrightarrow{b^{-1}} & \overline{ft^2(3,4)} & \xrightarrow{a^{-1}} & \overline{t(2,1)} & \xrightarrow{b} & \overline{t^2(2,4)} & \xrightarrow{a} & \overline{ft(3,1)} & \xrightarrow{a} & \overline{t^2(4,4)} \\
& \xrightarrow{b^{-1}} & \overline{t(1,4)} & \xrightarrow{a} & \overline{ft^2(2,1)} & \xrightarrow{b^{-1}} & \overline{ft(1,0)} & \xrightarrow{a^{-1}} & \overline{t^2(0,0)} & \xrightarrow{a^{-1}} & \overline{ft(4,0)} \\
& \xrightarrow{a^{-1}} & \overline{t^2(3,0)} & \xrightarrow{a^{-1}} & \overline{ft(2,0)} & \xrightarrow{a^{-1}} & \overline{t^2(1,0)} & \xrightarrow{a^{-1}} & \overline{ft(0,0)} & \xrightarrow{a^{-1}} & \overline{t^2(4,0)} \\
& \xrightarrow{a^{-1}} & \overline{ft(3,0)} & \xrightarrow{a^{-1}} & \overline{t^2(2,0)} & \xrightarrow{b^{-1}} & \overline{t(4,3)} & \xrightarrow{b^{-1}} & \overline{(4,2)} & \xrightarrow{a} & \overline{f(0,3)} \\
& \xrightarrow{a} & \overline{(1,2)} & \xrightarrow{a} & \overline{f(2,3)} & \xrightarrow{a} & \overline{(3,2)} & \xrightarrow{a} & \overline{f(4,3)} & \xrightarrow{a} & \overline{(0,2)} \\
& \xrightarrow{a} & \overline{f(1,3)} & \xrightarrow{a} & \overline{(2,2)} & \xrightarrow{a} & \overline{f(3,3)} & \xrightarrow{b^{-1}} & \overline{ft^2(2,3)} & \xrightarrow{a^{-1}} & \overline{t(1,2)} \\
& \xrightarrow{a^{-1}} & \overline{ft^2(0,3)} & \xrightarrow{b^{-1}} & \overline{ft(1,1)} & \xrightarrow{a^{-1}} & \overline{t^2(0,4)} & \xrightarrow{a^{-1}} & \overline{ft(4,1)} & \xrightarrow{a^{-1}} & \overline{t^2(3,4)} \\
& \xrightarrow{a^{-1}} & \overline{ft(2,1)} & \xrightarrow{a^{-1}} & \overline{t^2(1,4)} & \xrightarrow{a^{-1}} & \overline{ft(0,1)} & \xrightarrow{b} & \overline{ft^2(3,2)} & \xrightarrow{a^{-1}} & \overline{t(2,3)} \\
& \xrightarrow{b} & \overline{t^2(3,3)} & \xrightarrow{a^{-1}} & \overline{ft(2,2)} & \xrightarrow{a^{-1}} & \overline{t^2(1,3)} & \xrightarrow{b^{-1}} & \overline{t(3,0)} & \xrightarrow{a^{-1}} & \overline{ft^2(2,0)} \\
& \xrightarrow{a^{-1}} & \overline{t(1,0)} & \xrightarrow{a^{-1}} & \overline{ft^2(0,0)} & \xrightarrow{a^{-1}} & \overline{t(4,0)} & \xrightarrow{a^{-1}} & \overline{ft^2(3,0)} & \xrightarrow{a^{-1}} & \overline{t(2,0)} \\
& \xrightarrow{b^{-1}} & \overline{(4,3)} & \xrightarrow{a} & \overline{f(0,2)} & \xrightarrow{a} & \overline{(1,3)} & \xrightarrow{a} & \overline{f(2,2)} & \xrightarrow{a} & \overline{(3,3)} \\
& \xrightarrow{a} & \overline{f(4,2)} & \xrightarrow{a} & \overline{(0,3)} & \xrightarrow{a} & \overline{f(1,2)} & \xrightarrow{a} & \overline{(2,3)} & \xrightarrow{a} & \overline{f(3,2)} \\
& \xrightarrow{b^{-1}} & \overline{ft^2(0,1)} & \xrightarrow{a^{-1}} & \overline{t(4,4)} & \xrightarrow{a^{-1}} & \overline{ft^2(3,1)} & \xrightarrow{a^{-1}} & \overline{t(2,4)} & \xrightarrow{a^{-1}} & \overline{ft^2(1,1)} \\
& \xrightarrow{a^{-1}} & \overline{t(0,4)} & \xrightarrow{a^{-1}} & \overline{ft^2(4,1)} & \xrightarrow{b^{-1}} & \overline{ft(0,3)} & \xrightarrow{a^{-1}} & \overline{t^2(4,2)} & \xrightarrow{a^{-1}} & \overline{ft(3,3)} \\
& \xrightarrow{b} & \overline{ft^2(0,4)} & \xrightarrow{a^{-1}} & \overline{t(4,1)} & \xrightarrow{b} & \overline{t^2(1,1)} & \xrightarrow{a^{-1}} & \overline{ft(0,4)} & \xrightarrow{a^{-1}} & \overline{t^2(4,1)} \\
& \xrightarrow{a^{-1}} & \overline{ft(3,4)} & \xrightarrow{a^{-1}} & \overline{t^2(2,1)} & \xrightarrow{a^{-1}} & \overline{ft(1,4)} & \xrightarrow{a^{-1}} & \overline{t^2(0,1)} & \xrightarrow{a^{-1}} & \overline{ft(4,4)} \\
& \xrightarrow{b} & \overline{ft^2(0,2)} & \xrightarrow{a} & \overline{t(1,3)} & \xrightarrow{b} & \overline{t^2(1,2)} & \xrightarrow{a} & \overline{ft(2,3)} & \xrightarrow{a} & \overline{t^2(3,2)} \\
& \xrightarrow{a} & \overline{ft(4,3)} & \xrightarrow{a} & \overline{t^2(0,2)} & \xrightarrow{a} & \overline{ft(1,3)} & \xrightarrow{a} & \overline{t^2(2,2)} & \xrightarrow{b^{-1}} & \overline{t(3,2)} \\
& \xrightarrow{a} & \overline{ft^2(4,3)} & \xrightarrow{b^{-1}} & \overline{ft(4,2)} & \xrightarrow{a} & \overline{t^2(0,3)} & \xrightarrow{a} & \overline{ft(1,2)} & \xrightarrow{a} & \overline{t^2(2,3)} \\
& \xrightarrow{a} & \overline{ft(3,2)} & \xrightarrow{b} & \overline{ft^2(2,2)} & \xrightarrow{a} & \overline{t(3,3)} & \xrightarrow{a} & \overline{ft^2(4,2)} & \xrightarrow{a} & \overline{t(0,3)} \\
& \xrightarrow{a} & \overline{ft^2(1,2)} & \xrightarrow{b} & \overline{f(3,0)} & \xrightarrow{a^{-1}} & \overline{(2,0)} & \xrightarrow{a^{-1}} & \overline{f(1,0)} & \xrightarrow{a^{-1}} & \overline{(0,0)}
\end{array}
$$

$f$ inverts $t$, $t$ is nontrivial on $P$, and $S = \{f(1,1), t\}$

$$\begin{array}{lllllll}
\overline{(0,0)} & \xrightarrow{b^{-1}} \overline{t^2(0,0)} & \xrightarrow{a} \overline{ft(1,1)} & \xrightarrow{b^{-1}} \overline{f(4,1)} & \xrightarrow{b^{-1}} \overline{ft^2(0,3)} & \xrightarrow{a^{-1}} \overline{t(4,3)} \\
& \xrightarrow{b^{-1}} \overline{(4,2)} & \xrightarrow{b^{-1}} \overline{t^2(2,0)} & \xrightarrow{a} \overline{ft(3,1)} & \xrightarrow{b^{-1}} \overline{f(3,4)} & \xrightarrow{b^{-1}} \overline{ft^2(4,0)} \\
& \xrightarrow{a^{-1}} \overline{t(3,1)} & \xrightarrow{b^{-1}} \overline{(3,4)} & \xrightarrow{b^{-1}} \overline{t^2(4,0)} & \xrightarrow{a} \overline{ft(0,1)} & \xrightarrow{b^{-1}} \overline{f(2,2)} \\
& \xrightarrow{b^{-1}} \overline{ft^2(3,2)} & \xrightarrow{a} \overline{t(4,4)} & \xrightarrow{b^{-1}} \overline{(1,4)} & \xrightarrow{b^{-1}} \overline{t^2(0,2)} & \xrightarrow{a} \overline{ft(1,4)} \\
& \xrightarrow{b^{-1}} \overline{f(0,2)} & \xrightarrow{b^{-1}} \overline{ft^2(4,4)} & \xrightarrow{a^{-1}} \overline{t(3,2)} & \xrightarrow{b^{-1}} \overline{(0,1)} & \xrightarrow{b^{-1}} \overline{t^2(2,2)} \\
& \xrightarrow{a} \overline{ft(3,4)} & \xrightarrow{b^{-1}} \overline{f(4,0)} & \xrightarrow{b^{-1}} \overline{ft^2(3,1)} & \xrightarrow{a^{-1}} \overline{t(2,0)} & \xrightarrow{b^{-1}} \overline{(4,3)} \\
& \xrightarrow{b^{-1}} \overline{t^2(4,2)} & \xrightarrow{a} \overline{ft(0,4)} & \xrightarrow{b^{-1}} \overline{f(3,3)} & \xrightarrow{b^{-1}} \overline{ft^2(2,3)} & \xrightarrow{a^{-1}} \overline{t(1,3)} \\
& \xrightarrow{b^{-1}} \overline{(3,0)} & \xrightarrow{b^{-1}} \overline{t^2(1,2)} & \xrightarrow{a} \overline{ft(2,4)} & \xrightarrow{b^{-1}} \overline{f(2,1)} & \xrightarrow{b^{-1}} \overline{ft^2(1,0)} \\
& \xrightarrow{a^{-1}} \overline{t(0,1)} & \xrightarrow{b^{-1}} \overline{(2,2)} & \xrightarrow{b^{-1}} \overline{t^2(3,2)} & \xrightarrow{a} \overline{ft(4,4)} & \xrightarrow{b^{-1}} \overline{f(1,4)} \\
& \xrightarrow{b^{-1}} \overline{ft^2(0,2)} & \xrightarrow{a} \overline{t(1,4)} & \xrightarrow{b^{-1}} \overline{(0,2)} & \xrightarrow{b^{-1}} \overline{t^2(4,4)} & \xrightarrow{a} \overline{ft(0,2)} \\
& \xrightarrow{b^{-1}} \overline{f(4,4)} & \xrightarrow{b^{-1}} \overline{ft^2(1,4)} & \xrightarrow{a^{-1}} \overline{t(0,2)} & \xrightarrow{b^{-1}} \overline{(4,4)} & \xrightarrow{b^{-1}} \overline{t^2(1,4)} \\
& \xrightarrow{a} \overline{ft(2,2)} & \xrightarrow{b^{-1}} \overline{f(3,2)} & \xrightarrow{b^{-1}} \overline{ft^2(0,1)} & \xrightarrow{a^{-1}} \overline{t(4,0)} & \xrightarrow{b^{-1}} \overline{(3,1)} \\
& \xrightarrow{b^{-1}} \overline{t^2(3,4)} & \xrightarrow{a} \overline{ft(4,2)} & \xrightarrow{b^{-1}} \overline{f(2,0)} & \xrightarrow{b^{-1}} \overline{ft^2(4,3)} & \xrightarrow{a^{-1}} \overline{t(3,3)} \\
& \xrightarrow{b^{-1}} \overline{(2,3)} & \xrightarrow{b^{-1}} \overline{t^2(0,4)} & \xrightarrow{a} \overline{ft(1,2)} & \xrightarrow{b^{-1}} \overline{f(1,3)} & \xrightarrow{b^{-1}} \overline{ft^2(3,0)} \\
& \xrightarrow{a^{-1}} \overline{t(2,1)} & \xrightarrow{b^{-1}} \overline{(1,0)} & \xrightarrow{b^{-1}} \overline{t^2(2,4)} & \xrightarrow{a} \overline{ft(3,2)} & \xrightarrow{b^{-1}} \overline{f(0,1)} \\
& \xrightarrow{b^{-1}} \overline{ft^2(2,2)} & \xrightarrow{a} \overline{t(3,4)} & \xrightarrow{b^{-1}} \overline{(4,0)} & \xrightarrow{b^{-1}} \overline{t^2(3,1)} & \xrightarrow{a} \overline{ft(4,0)} \\
& \xrightarrow{b^{-1}} \overline{f(3,1)} & \xrightarrow{b^{-1}} \overline{ft^2(3,4)} & \xrightarrow{a^{-1}} \overline{t(2,2)} & \xrightarrow{b^{-1}} \overline{(3,2)} & \xrightarrow{b^{-1}} \overline{t^2(0,1)} \\
& \xrightarrow{a} \overline{ft(1,0)} & \xrightarrow{b^{-1}} \overline{f(2,4)} & \xrightarrow{b^{-1}} \overline{ft^2(2,1)} & \xrightarrow{a^{-1}} \overline{t(1,0)} & \xrightarrow{b^{-1}} \overline{(2,4)} \\
& \xrightarrow{b^{-1}} \overline{t^2(2,1)} & \xrightarrow{a} \overline{ft(3,0)} & \xrightarrow{b^{-1}} \overline{f(1,2)} & \xrightarrow{b^{-1}} \overline{ft^2(1,3)} & \xrightarrow{a^{-1}} \overline{t(0,3)} \\
& \xrightarrow{b^{-1}} \overline{(1,1)} & \xrightarrow{b^{-1}} \overline{t^2(4,1)} & \xrightarrow{a} \overline{ft(0,0)} & \xrightarrow{b^{-1}} \overline{f(0,0)} & \xrightarrow{b^{-1}} \overline{ft^2(0,0)} \\
& \xrightarrow{a^{-1}} \overline{t(4,1)} & \xrightarrow{b^{-1}} \overline{(0,3)} & \xrightarrow{b^{-1}} \overline{t^2(1,1)} & \xrightarrow{a} \overline{ft(2,0)} & \xrightarrow{b^{-1}} \overline{f(4,3)} \\
& \xrightarrow{b^{-1}} \overline{ft^2(4,2)} & \xrightarrow{a} \overline{t(0,4)} & \xrightarrow{b^{-1}} \overline{(3,3)} & \xrightarrow{b^{-1}} \overline{t^2(2,3)} & \xrightarrow{a} \overline{ft(3,3)} \\
& \xrightarrow{b^{-1}} \overline{f(2,3)} & \xrightarrow{b^{-1}} \overline{ft^2(0,4)} & \xrightarrow{a^{-1}} \overline{t(4,2)} & \xrightarrow{b^{-1}} \overline{(2,0)} & \xrightarrow{b^{-1}} \overline{t^2(4,3)} \\
& \xrightarrow{a} \overline{ft(0,3)} & \xrightarrow{b^{-1}} \overline{f(1,1)} & \xrightarrow{b^{-1}} \overline{ft^2(4,1)} & \xrightarrow{a^{-1}} \overline{t(3,0)} & \xrightarrow{b^{-1}} \overline{(1,2)} \\
& \xrightarrow{b^{-1}} \overline{t^2(1,3)} & \xrightarrow{a} \overline{ft(2,3)} & \xrightarrow{b^{-1}} \overline{f(0,4)} & \xrightarrow{b^{-1}} \overline{ft^2(3,3)} & \xrightarrow{a^{-1}} \overline{t(2,3)} \\
& \xrightarrow{b^{-1}} \overline{(0,4)} & \xrightarrow{b^{-1}} \overline{t^2(3,3)} & \xrightarrow{a} \overline{ft(4,3)} & \xrightarrow{b^{-1}} \overline{f(4,2)} & \xrightarrow{b^{-1}} \overline{ft^2(2,0)} \\
& \xrightarrow{a^{-1}} \overline{t(1,1)} & \xrightarrow{b^{-1}} \overline{(4,1)} & \xrightarrow{b^{-1}} \overline{t^2(0,3)} & \xrightarrow{a} \overline{ft(1,3)} & \xrightarrow{b^{-1}} \overline{f(3,0)} \\
& \xrightarrow{b^{-1}} \overline{ft^2(1,2)} & \xrightarrow{a} \overline{t(2,4)} & \xrightarrow{b^{-1}} \overline{(2,1)} & \xrightarrow{b^{-1}} \overline{t^2(1,0)} & \xrightarrow{a} \overline{ft(2,1)} \\
& \xrightarrow{b^{-1}} \overline{f(1,0)} & \xrightarrow{b^{-1}} \overline{ft^2(2,4)} & \xrightarrow{a^{-1}} \overline{t(1,2)} & \xrightarrow{b^{-1}} \overline{(1,3)} & \xrightarrow{b^{-1}} \overline{t^2(3,0)} \\
& \xrightarrow{a} \overline{ft(4,1)} & \xrightarrow{b^{-1}} \overline{f(0,3)} & \xrightarrow{b^{-1}} \overline{ft^2(1,1)} & \xrightarrow{a^{-1}} \overline{t(0,0)} & \xrightarrow{b^{-1}} \overline{(0,0)}
\end{array}$$

$f$ inverts $t$, $t$ is nontrivial on $P$, and $S = \{f(1,2), t\}$

$$\overline{(0,0)} \xrightarrow{b^{-1}} \overline{t^2(0,0)} \xrightarrow{a} \overline{ft(1,2)} \xrightarrow{b^{-1}} \overline{f(1,3)} \xrightarrow{b^{-1}} \overline{ft^2(3,0)} \xrightarrow{a^{-1}} \overline{t(2,2)}$$
$$\xrightarrow{b^{-1}} \overline{(3,2)} \xrightarrow{b^{-1}} \overline{t^2(0,1)} \xrightarrow{a} \overline{ft(1,1)} \xrightarrow{b^{-1}} \overline{f(4,1)} \xrightarrow{b^{-1}} \overline{ft^2(0,3)}$$
$$\xrightarrow{a^{-1}} \overline{t(4,4)} \xrightarrow{b^{-1}} \overline{(1,4)} \xrightarrow{b^{-1}} \overline{t^2(0,2)} \xrightarrow{a} \overline{ft(1,0)} \xrightarrow{b^{-1}} \overline{f(2,4)}$$
$$\xrightarrow{b^{-1}} \overline{ft^2(2,1)} \xrightarrow{a^{-1}} \overline{t(1,1)} \xrightarrow{b^{-1}} \overline{(4,1)} \xrightarrow{b^{-1}} \overline{t^2(0,3)} \xrightarrow{a} \overline{ft(1,4)}$$
$$\xrightarrow{b^{-1}} \overline{f(0,2)} \xrightarrow{b^{-1}} \overline{ft^2(4,4)} \xrightarrow{a^{-1}} \overline{t(3,3)} \xrightarrow{b^{-1}} \overline{(2,3)} \xrightarrow{b^{-1}} \overline{t^2(0,4)}$$
$$\xrightarrow{a^{-1}} \overline{ft(4,3)} \xrightarrow{b^{-1}} \overline{f(4,2)} \xrightarrow{b^{-1}} \overline{ft^2(2,0)} \xrightarrow{a^{-1}} \overline{t(1,2)} \xrightarrow{b^{-1}} \overline{(1,3)}$$
$$\xrightarrow{b^{-1}} \overline{t^2(3,0)} \xrightarrow{a} \overline{ft(4,2)} \xrightarrow{b^{-1}} \overline{f(2,0)} \xrightarrow{b^{-1}} \overline{ft^2(4,3)} \xrightarrow{a^{-1}} \overline{t(3,4)}$$
$$\xrightarrow{b^{-1}} \overline{(4,0)} \xrightarrow{b^{-1}} \overline{t^2(3,1)} \xrightarrow{a} \overline{ft(4,1)} \xrightarrow{b^{-1}} \overline{f(0,3)} \xrightarrow{b^{-1}} \overline{ft^2(1,1)}$$
$$\xrightarrow{a^{-1}} \overline{t(0,1)} \xrightarrow{b^{-1}} \overline{(2,2)} \xrightarrow{b^{-1}} \overline{t^2(3,2)} \xrightarrow{a} \overline{ft(4,0)} \xrightarrow{b^{-1}} \overline{f(3,1)}$$
$$\xrightarrow{b^{-1}} \overline{ft^2(3,4)} \xrightarrow{a^{-1}} \overline{t(2,3)} \xrightarrow{b^{-1}} \overline{(0,4)} \xrightarrow{b^{-1}} \overline{t^2(3,3)} \xrightarrow{a} \overline{ft(4,4)}$$
$$\xrightarrow{b^{-1}} \overline{f(1,4)} \xrightarrow{b^{-1}} \overline{ft^2(0,2)} \xrightarrow{a^{-1}} \overline{t(4,0)} \xrightarrow{b^{-1}} \overline{(3,1)} \xrightarrow{b^{-1}} \overline{t^2(3,4)}$$
$$\xrightarrow{a^{-1}} \overline{ft(2,3)} \xrightarrow{b^{-1}} \overline{f(0,4)} \xrightarrow{b^{-1}} \overline{ft^2(3,3)} \xrightarrow{a^{-1}} \overline{t(2,4)} \xrightarrow{b^{-1}} \overline{(2,1)}$$
$$\xrightarrow{b^{-1}} \overline{t^2(1,0)} \xrightarrow{a} \overline{ft(2,2)} \xrightarrow{b^{-1}} \overline{f(3,2)} \xrightarrow{b^{-1}} \overline{ft^2(0,1)} \xrightarrow{a^{-1}} \overline{t(4,1)}$$
$$\xrightarrow{b^{-1}} \overline{(0,3)} \xrightarrow{b^{-1}} \overline{t^2(1,1)} \xrightarrow{a} \overline{ft(2,1)} \xrightarrow{b^{-1}} \overline{f(1,0)} \xrightarrow{b^{-1}} \overline{ft^2(2,4)}$$
$$\xrightarrow{a^{-1}} \overline{t(1,3)} \xrightarrow{b^{-1}} \overline{(3,0)} \xrightarrow{b^{-1}} \overline{t^2(1,2)} \xrightarrow{a} \overline{ft(2,0)} \xrightarrow{b^{-1}} \overline{f(4,3)}$$
$$\xrightarrow{b^{-1}} \overline{ft^2(4,2)} \xrightarrow{a^{-1}} \overline{t(3,0)} \xrightarrow{b^{-1}} \overline{(1,2)} \xrightarrow{b^{-1}} \overline{t^2(1,3)} \xrightarrow{a} \overline{ft(2,4)}$$
$$\xrightarrow{b^{-1}} \overline{f(2,1)} \xrightarrow{b^{-1}} \overline{ft^2(1,0)} \xrightarrow{a^{-1}} \overline{t(0,2)} \xrightarrow{b^{-1}} \overline{(4,4)} \xrightarrow{b^{-1}} \overline{t^2(1,4)}$$
$$\xrightarrow{a^{-1}} \overline{ft(0,3)} \xrightarrow{b^{-1}} \overline{f(1,1)} \xrightarrow{b^{-1}} \overline{ft^2(4,1)} \xrightarrow{a^{-1}} \overline{t(3,1)} \xrightarrow{b^{-1}} \overline{(3,4)}$$
$$\xrightarrow{b^{-1}} \overline{t^2(4,0)} \xrightarrow{a} \overline{ft(0,2)} \xrightarrow{b^{-1}} \overline{f(4,4)} \xrightarrow{b^{-1}} \overline{ft^2(1,4)} \xrightarrow{a^{-1}} \overline{t(0,3)}$$
$$\xrightarrow{b^{-1}} \overline{(1,1)} \xrightarrow{b^{-1}} \overline{t^2(4,1)} \xrightarrow{a} \overline{ft(0,1)} \xrightarrow{b^{-1}} \overline{f(2,2)} \xrightarrow{b^{-1}} \overline{ft^2(3,2)}$$
$$\xrightarrow{a^{-1}} \overline{t(2,0)} \xrightarrow{b^{-1}} \overline{(4,3)} \xrightarrow{b^{-1}} \overline{t^2(4,2)} \xrightarrow{a} \overline{ft(0,0)} \xrightarrow{b^{-1}} \overline{f(0,0)}$$
$$\xrightarrow{b^{-1}} \overline{ft^2(0,0)} \xrightarrow{a^{-1}} \overline{t(4,2)} \xrightarrow{b^{-1}} \overline{(2,0)} \xrightarrow{b^{-1}} \overline{t^2(4,3)} \xrightarrow{a} \overline{ft(0,4)}$$
$$\xrightarrow{b^{-1}} \overline{f(3,3)} \xrightarrow{b^{-1}} \overline{ft^2(2,3)} \xrightarrow{a^{-1}} \overline{t(1,4)} \xrightarrow{b^{-1}} \overline{(0,2)} \xrightarrow{b^{-1}} \overline{t^2(4,4)}$$
$$\xrightarrow{a^{-1}} \overline{ft(3,3)} \xrightarrow{b^{-1}} \overline{f(2,3)} \xrightarrow{b^{-1}} \overline{ft^2(0,4)} \xrightarrow{a^{-1}} \overline{t(4,3)} \xrightarrow{b^{-1}} \overline{(4,2)}$$
$$\xrightarrow{b^{-1}} \overline{t^2(2,0)} \xrightarrow{a} \overline{ft(3,2)} \xrightarrow{b^{-1}} \overline{f(0,1)} \xrightarrow{b^{-1}} \overline{ft^2(2,2)} \xrightarrow{a^{-1}} \overline{t(1,0)}$$
$$\xrightarrow{b^{-1}} \overline{(2,4)} \xrightarrow{b^{-1}} \overline{t^2(2,1)} \xrightarrow{a} \overline{ft(3,1)} \xrightarrow{b^{-1}} \overline{f(3,4)} \xrightarrow{b^{-1}} \overline{ft^2(4,0)}$$
$$\xrightarrow{a^{-1}} \overline{t(3,2)} \xrightarrow{b^{-1}} \overline{(0,1)} \xrightarrow{b^{-1}} \overline{t^2(2,2)} \xrightarrow{a} \overline{ft(3,0)} \xrightarrow{b^{-1}} \overline{f(1,2)}$$
$$\xrightarrow{b^{-1}} \overline{ft^2(1,3)} \xrightarrow{a^{-1}} \overline{t(0,4)} \xrightarrow{b^{-1}} \overline{(3,3)} \xrightarrow{b^{-1}} \overline{t^2(2,3)} \xrightarrow{a} \overline{ft(3,4)}$$
$$\xrightarrow{b^{-1}} \overline{f(4,0)} \xrightarrow{b^{-1}} \overline{ft^2(3,1)} \xrightarrow{a^{-1}} \overline{t(2,1)} \xrightarrow{b^{-1}} \overline{(1,0)} \xrightarrow{b^{-1}} \overline{t^2(2,4)}$$
$$\xrightarrow{a^{-1}} \overline{ft(1,3)} \xrightarrow{b^{-1}} \overline{f(3,0)} \xrightarrow{b^{-1}} \overline{ft^2(1,2)} \xrightarrow{a^{-1}} \overline{t(0,0)} \xrightarrow{b^{-1}} \overline{(0,0)}$$

$f$ inverts $t$, $t$ is nontrivial on $P$, and $S = \{f(0,1), t\}$

$$\overline{(0,0)} \xrightarrow{b} \overline{t(0,0)} \xrightarrow{b} \overline{t^2(0,0)} \xrightarrow{a} \overline{ft(0,1)} \xrightarrow{b} \overline{ft^2(3,2)} \xrightarrow{b} \overline{f(2,2)}$$
$$\xrightarrow{a} \overline{(2,4)} \xrightarrow{b^{-1}} \overline{t^2(2,1)} \xrightarrow{b^{-1}} \overline{t(1,0)} \xrightarrow{a} \overline{ft^2(1,1)} \xrightarrow{b^{-1}} \overline{ft(4,1)}$$
$$\xrightarrow{b^{-1}} \overline{f(0,3)} \xrightarrow{a} \overline{(0,3)} \xrightarrow{b} \overline{t(4,1)} \xrightarrow{b} \overline{t^2(1,1)} \xrightarrow{a} \overline{ft(1,0)}$$
$$\xrightarrow{b} \overline{ft^2(2,1)} \xrightarrow{b} \overline{f(2,4)} \xrightarrow{a} \overline{(2,2)} \xrightarrow{b} \overline{t(0,1)} \xrightarrow{b} \overline{t^2(3,2)}$$
$$\xrightarrow{a} \overline{ft(3,4)} \xrightarrow{b} \overline{ft^2(3,1)} \xrightarrow{b} \overline{f(4,0)} \xrightarrow{a} \overline{(4,1)} \xrightarrow{b^{-1}} \overline{t^2(0,3)}$$
$$\xrightarrow{b^{-1}} \overline{t(1,1)} \xrightarrow{a} \overline{ft^2(1,0)} \xrightarrow{b} \overline{f(2,1)} \xrightarrow{b} \overline{ft(2,4)} \xrightarrow{a} \overline{t^2(2,2)}$$
$$\xrightarrow{b^{-1}} \overline{t(3,2)} \xrightarrow{b^{-1}} \overline{(0,1)} \xrightarrow{a} \overline{f(0,0)} \xrightarrow{b^{-1}} \overline{ft^2(0,0)} \xrightarrow{b^{-1}} \overline{ft(0,0)}$$
$$\xrightarrow{a} \overline{t^2(0,1)} \xrightarrow{b^{-1}} \overline{t(2,2)} \xrightarrow{b^{-1}} \overline{(3,2)} \xrightarrow{a} \overline{f(3,4)} \xrightarrow{b^{-1}} \overline{ft^2(4,0)}$$
$$\xrightarrow{b^{-1}} \overline{ft(3,1)} \xrightarrow{a} \overline{t^2(3,0)} \xrightarrow{b} \overline{(1,3)} \xrightarrow{b} \overline{t(1,2)} \xrightarrow{a} \overline{ft^2(1,4)}$$
$$\xrightarrow{b} \overline{f(4,4)} \xrightarrow{b} \overline{ft(0,2)} \xrightarrow{a} \overline{t^2(0,4)} \xrightarrow{b^{-1}} \overline{t(3,3)} \xrightarrow{b^{-1}} \overline{(2,3)}$$
$$\xrightarrow{a} \overline{f(2,3)} \xrightarrow{b^{-1}} \overline{ft^2(0,4)} \xrightarrow{b^{-1}} \overline{ft(3,3)} \xrightarrow{a} \overline{t^2(3,3)} \xrightarrow{b^{-1}} \overline{t(2,3)}$$
$$\xrightarrow{b^{-1}} \overline{(0,4)} \xrightarrow{a} \overline{f(0,2)} \xrightarrow{b} \overline{ft(1,4)} \xrightarrow{b} \overline{ft^2(4,4)} \xrightarrow{a} \overline{t(4,2)}$$
$$\xrightarrow{b^{-1}} \overline{(2,0)} \xrightarrow{b^{-1}} \overline{t^2(4,3)} \xrightarrow{a} \overline{ft(4,3)} \xrightarrow{b} \overline{ft^2(2,0)} \xrightarrow{b} \overline{f(4,2)}$$
$$\xrightarrow{a} \overline{(4,4)} \xrightarrow{b} \overline{t(0,2)} \xrightarrow{b} \overline{t^2(1,4)} \xrightarrow{a} \overline{ft(1,2)} \xrightarrow{b^{-1}} \overline{f(1,3)}$$
$$\xrightarrow{b^{-1}} \overline{ft^2(3,0)} \xrightarrow{a} \overline{t(3,1)} \xrightarrow{b} \overline{t^2(4,0)} \xrightarrow{b} \overline{(3,4)} \xrightarrow{a} \overline{f(3,2)}$$
$$\xrightarrow{b^{-1}} \overline{ft^2(0,1)} \xrightarrow{b^{-1}} \overline{ft(2,2)} \xrightarrow{a} \overline{t^2(2,4)} \xrightarrow{b^{-1}} \overline{t(2,1)} \xrightarrow{b^{-1}} \overline{(1,0)}$$
$$\xrightarrow{a} \overline{f(1,1)} \xrightarrow{b} \overline{ft(0,3)} \xrightarrow{b} \overline{ft^2(4,1)} \xrightarrow{a} \overline{t(4,0)} \xrightarrow{b} \overline{t^2(3,4)}$$
$$\xrightarrow{b} \overline{(3,1)} \xrightarrow{a} \overline{f(3,0)} \xrightarrow{b^{-1}} \overline{ft^2(1,2)} \xrightarrow{b^{-1}} \overline{ft(1,3)} \xrightarrow{a} \overline{t^2(1,3)}$$
$$\xrightarrow{b^{-1}} \overline{t(3,0)} \xrightarrow{b^{-1}} \overline{(1,2)} \xrightarrow{a} \overline{f(1,4)} \xrightarrow{b^{-1}} \overline{ft^2(0,2)} \xrightarrow{b^{-1}} \overline{ft(4,4)}$$
$$\xrightarrow{a} \overline{t^2(4,2)} \xrightarrow{b^{-1}} \overline{t(2,0)} \xrightarrow{b^{-1}} \overline{(4,3)} \xrightarrow{a} \overline{f(4,3)} \xrightarrow{b} \overline{ft(2,0)}$$
$$\xrightarrow{b} \overline{ft^2(4,2)} \xrightarrow{a} \overline{t(4,4)} \xrightarrow{b^{-1}} \overline{(1,4)} \xrightarrow{b^{-1}} \overline{t^2(0,2)} \xrightarrow{a} \overline{ft(0,4)}$$
$$\xrightarrow{b} \overline{ft^2(2,3)} \xrightarrow{b} \overline{f(3,3)} \xrightarrow{a} \overline{(3,3)} \xrightarrow{b} \overline{t(0,4)} \xrightarrow{b} \overline{t^2(2,3)}$$
$$\xrightarrow{a} \overline{ft(2,3)} \xrightarrow{b} \overline{ft^2(3,3)} \xrightarrow{b} \overline{f(0,4)} \xrightarrow{a} \overline{(0,2)} \xrightarrow{b} \overline{t(1,4)}$$
$$\xrightarrow{b} \overline{t^2(4,4)} \xrightarrow{a} \overline{ft(4,2)} \xrightarrow{b^{-1}} \overline{f(2,0)} \xrightarrow{b^{-1}} \overline{ft^2(4,3)} \xrightarrow{a} \overline{t(4,3)}$$
$$\xrightarrow{b^{-1}} \overline{(4,2)} \xrightarrow{b^{-1}} \overline{t^2(2,0)} \xrightarrow{a} \overline{ft(2,1)} \xrightarrow{b} \overline{ft^2(2,4)} \xrightarrow{b} \overline{f(1,0)}$$
$$\xrightarrow{a} \overline{(1,1)} \xrightarrow{b} \overline{t(0,3)} \xrightarrow{b} \overline{t^2(4,1)} \xrightarrow{a} \overline{ft(4,0)} \xrightarrow{b} \overline{ft^2(3,4)}$$
$$\xrightarrow{b} \overline{f(3,1)} \xrightarrow{a} \overline{(3,0)} \xrightarrow{b^{-1}} \overline{t^2(1,2)} \xrightarrow{b^{-1}} \overline{t(1,3)} \xrightarrow{a} \overline{ft^2(1,3)}$$
$$\xrightarrow{b} \overline{f(1,2)} \xrightarrow{b} \overline{ft(3,0)} \xrightarrow{a} \overline{t^2(3,1)} \xrightarrow{b^{-1}} \overline{t(3,4)} \xrightarrow{b^{-1}} \overline{(4,0)}$$
$$\xrightarrow{a} \overline{f(4,1)} \xrightarrow{b^{-1}} \overline{ft^2(0,3)} \xrightarrow{b^{-1}} \overline{ft(1,1)} \xrightarrow{a} \overline{t^2(1,0)} \xrightarrow{b} \overline{(2,1)}$$
$$\xrightarrow{b} \overline{t(2,4)} \xrightarrow{a} \overline{ft^2(2,2)} \xrightarrow{b^{-1}} \overline{ft(3,2)} \xrightarrow{b^{-1}} \overline{f(0,1)} \xrightarrow{a} \overline{(0,0)}$$

$f$ inverts $t$, $t$ is nontrivial on $P$, and $S = \{f(1,0), ft(\lambda, 2\lambda)\}$ with $\lambda = 0$

$$\overline{(0,0)} \xrightarrow{a^{-1}} \overline{f(4,0)} \xrightarrow{a^{-1}} \overline{(3,0)} \xrightarrow{a^{-1}} \overline{f(2,0)} \xrightarrow{a^{-1}} \overline{(1,0)} \xrightarrow{a^{-1}} \overline{f(0,0)}$$
$$\xrightarrow{a^{-1}} \overline{(4,0)} \xrightarrow{b} \overline{ft(3,4)} \xrightarrow{a^{-1}} \overline{t^2(2,1)} \xrightarrow{a^{-1}} \overline{ft(1,4)} \xrightarrow{a^{-1}} \overline{t^2(0,1)}$$
$$\xrightarrow{a^{-1}} \overline{ft(4,4)} \xrightarrow{a^{-1}} \overline{t^2(3,1)} \xrightarrow{a^{-1}} \overline{ft(2,4)} \xrightarrow{a^{-1}} \overline{t^2(1,1)} \xrightarrow{a^{-1}} \overline{ft(0,4)}$$
$$\xrightarrow{a^{-1}} \overline{t^2(4,1)} \xrightarrow{b} \overline{ft^2(0,2)} \xrightarrow{a^{-1}} \overline{t(4,3)} \xrightarrow{a^{-1}} \overline{ft^2(3,2)} \xrightarrow{a^{-1}} \overline{t(2,3)}$$
$$\xrightarrow{a^{-1}} \overline{ft^2(1,2)} \xrightarrow{a^{-1}} \overline{t(0,3)} \xrightarrow{a^{-1}} \overline{ft^2(4,2)} \xrightarrow{a^{-1}} \overline{t(3,3)} \xrightarrow{b} \overline{f(2,2)}$$
$$\xrightarrow{a^{-1}} \overline{(1,3)} \xrightarrow{a^{-1}} \overline{f(0,2)} \xrightarrow{a^{-1}} \overline{(4,3)} \xrightarrow{b} \overline{ft(4,3)} \xrightarrow{a^{-1}} \overline{t^2(3,2)}$$
$$\xrightarrow{a^{-1}} \overline{ft(2,3)} \xrightarrow{a^{-1}} \overline{t^2(1,2)} \xrightarrow{a^{-1}} \overline{ft(0,3)} \xrightarrow{a^{-1}} \overline{t^2(4,2)} \xrightarrow{a^{-1}} \overline{ft(3,3)}$$
$$\xrightarrow{a^{-1}} \overline{t^2(2,2)} \xrightarrow{a^{-1}} \overline{ft(1,3)} \xrightarrow{a^{-1}} \overline{t^2(0,2)} \xrightarrow{b} \overline{ft^2(4,1)} \xrightarrow{a^{-1}} \overline{t(3,4)}$$
$$\xrightarrow{a^{-1}} \overline{ft^2(2,1)} \xrightarrow{a^{-1}} \overline{t(1,4)} \xrightarrow{a^{-1}} \overline{ft^2(0,1)} \xrightarrow{a^{-1}} \overline{t(4,4)} \xrightarrow{a^{-1}} \overline{ft^2(3,1)}$$
$$\xrightarrow{a^{-1}} \overline{t(2,4)} \xrightarrow{a^{-1}} \overline{ft^2(1,1)} \xrightarrow{a^{-1}} \overline{t(0,4)} \xrightarrow{b} \overline{f(3,2)} \xrightarrow{a^{-1}} \overline{(2,3)}$$
$$\xrightarrow{a^{-1}} \overline{f(1,2)} \xrightarrow{a^{-1}} \overline{(0,3)} \xrightarrow{a^{-1}} \overline{f(4,2)} \xrightarrow{a^{-1}} \overline{(3,3)} \xrightarrow{b} \overline{ft(2,2)}$$
$$\xrightarrow{a^{-1}} \overline{t^2(1,3)} \xrightarrow{b} \overline{ft^2(3,0)} \xrightarrow{a^{-1}} \overline{t(2,0)} \xrightarrow{a^{-1}} \overline{ft^2(1,0)} \xrightarrow{a^{-1}} \overline{t(0,0)}$$
$$\xrightarrow{a^{-1}} \overline{ft^2(4,0)} \xrightarrow{a^{-1}} \overline{t(3,0)} \xrightarrow{a^{-1}} \overline{ft^2(2,0)} \xrightarrow{a^{-1}} \overline{t(1,0)} \xrightarrow{b} \overline{f(2,1)}$$
$$\xrightarrow{a^{-1}} \overline{(1,4)} \xrightarrow{a^{-1}} \overline{f(0,1)} \xrightarrow{a^{-1}} \overline{(4,4)} \xrightarrow{b} \overline{ft(1,1)} \xrightarrow{a^{-1}} \overline{t^2(0,4)}$$
$$\xrightarrow{a^{-1}} \overline{ft(4,1)} \xrightarrow{a^{-1}} \overline{t^2(3,4)} \xrightarrow{a^{-1}} \overline{ft(2,1)} \xrightarrow{a^{-1}} \overline{t^2(1,4)} \xrightarrow{a^{-1}} \overline{ft(0,1)}$$
$$\xrightarrow{a^{-1}} \overline{t^2(4,4)} \xrightarrow{a^{-1}} \overline{ft(3,1)} \xrightarrow{a^{-1}} \overline{t^2(2,4)} \xrightarrow{b} \overline{ft^2(2,4)} \xrightarrow{a^{-1}} \overline{t(1,1)}$$
$$\xrightarrow{a^{-1}} \overline{ft^2(0,4)} \xrightarrow{a^{-1}} \overline{t(4,1)} \xrightarrow{a^{-1}} \overline{ft^2(3,4)} \xrightarrow{a^{-1}} \overline{t(2,1)} \xrightarrow{a^{-1}} \overline{ft^2(1,4)}$$
$$\xrightarrow{a^{-1}} \overline{t(0,1)} \xrightarrow{a^{-1}} \overline{ft^2(4,4)} \xrightarrow{a^{-1}} \overline{t(3,1)} \xrightarrow{b} \overline{f(3,1)} \xrightarrow{a^{-1}} \overline{(2,4)}$$
$$\xrightarrow{a^{-1}} \overline{f(1,1)} \xrightarrow{a^{-1}} \overline{(0,4)} \xrightarrow{a^{-1}} \overline{f(4,1)} \xrightarrow{a^{-1}} \overline{(3,4)} \xrightarrow{b} \overline{ft(4,0)}$$
$$\xrightarrow{a^{-1}} \overline{t^2(3,0)} \xrightarrow{b} \overline{ft^2(1,3)} \xrightarrow{a^{-1}} \overline{t(0,2)} \xrightarrow{a^{-1}} \overline{ft^2(4,3)} \xrightarrow{a^{-1}} \overline{t(3,2)}$$
$$\xrightarrow{a^{-1}} \overline{ft^2(2,3)} \xrightarrow{a^{-1}} \overline{t(1,2)} \xrightarrow{a^{-1}} \overline{ft^2(0,3)} \xrightarrow{a^{-1}} \overline{t(4,2)} \xrightarrow{a^{-1}} \overline{ft^2(3,3)}$$
$$\xrightarrow{a^{-1}} \overline{t(2,2)} \xrightarrow{b} \overline{f(3,3)} \xrightarrow{a^{-1}} \overline{(2,2)} \xrightarrow{a^{-1}} \overline{f(1,3)} \xrightarrow{a^{-1}} \overline{(0,2)}$$
$$\xrightarrow{a^{-1}} \overline{f(4,3)} \xrightarrow{a^{-1}} \overline{(3,2)} \xrightarrow{a^{-1}} \overline{f(2,3)} \xrightarrow{a^{-1}} \overline{(1,2)} \xrightarrow{a^{-1}} \overline{f(0,3)}$$
$$\xrightarrow{a^{-1}} \overline{(4,2)} \xrightarrow{b} \overline{ft(2,0)} \xrightarrow{a^{-1}} \overline{t^2(1,0)} \xrightarrow{a^{-1}} \overline{ft(0,0)} \xrightarrow{a^{-1}} \overline{t^2(4,0)}$$
$$\xrightarrow{a^{-1}} \overline{ft(3,0)} \xrightarrow{a^{-1}} \overline{t^2(2,0)} \xrightarrow{a^{-1}} \overline{ft(1,0)} \xrightarrow{a^{-1}} \overline{t^2(0,0)} \xrightarrow{b} \overline{ft^2(0,0)}$$
$$\xrightarrow{a^{-1}} \overline{t(4,0)} \xrightarrow{b} \overline{f(3,4)} \xrightarrow{a^{-1}} \overline{(2,1)} \xrightarrow{a^{-1}} \overline{f(1,4)} \xrightarrow{a^{-1}} \overline{(0,1)}$$
$$\xrightarrow{a^{-1}} \overline{f(4,4)} \xrightarrow{a^{-1}} \overline{(3,1)} \xrightarrow{a^{-1}} \overline{f(2,4)} \xrightarrow{a^{-1}} \overline{(1,1)} \xrightarrow{a^{-1}} \overline{f(0,4)}$$
$$\xrightarrow{a^{-1}} \overline{(4,1)} \xrightarrow{b} \overline{ft(0,2)} \xrightarrow{a^{-1}} \overline{t^2(4,3)} \xrightarrow{a^{-1}} \overline{ft(3,2)} \xrightarrow{a^{-1}} \overline{t^2(2,3)}$$
$$\xrightarrow{a^{-1}} \overline{ft(1,2)} \xrightarrow{a^{-1}} \overline{t^2(0,3)} \xrightarrow{a^{-1}} \overline{ft(4,2)} \xrightarrow{a^{-1}} \overline{t^2(3,3)} \xrightarrow{b} \overline{ft^2(2,2)}$$
$$\xrightarrow{a^{-1}} \overline{t(1,3)} \xrightarrow{b} \overline{f(3,0)} \xrightarrow{a^{-1}} \overline{(2,0)} \xrightarrow{a^{-1}} \overline{f(1,0)} \xrightarrow{a^{-1}} \overline{(0,0)}$$

$f$ inverts $t$, $t$ is nontrivial on $P$, and $S = \{f(1,0), ft(\lambda, 2\lambda)\}$ with $\lambda = 1$

$$
\begin{array}{ccccccccccc}
\overline{(0,0)} & \xrightarrow{a^{-1}} & \overline{f(4,0)} & \xrightarrow{a^{-1}} & \overline{(3,0)} & \xrightarrow{a^{-1}} & \overline{f(2,0)} & \xrightarrow{a^{-1}} & \overline{(1,0)} & \xrightarrow{a^{-1}} & \overline{f(0,0)} \\
 & \xrightarrow{a^{-1}} & \overline{(4,0)} & \xrightarrow{b} & \overline{ft(4,1)} & \xrightarrow{a} & \overline{t^2(0,4)} & \xrightarrow{a} & \overline{ft(1,1)} & \xrightarrow{a} & \overline{t^2(2,4)} \\
 & \xrightarrow{a} & \overline{ft(3,1)} & \xrightarrow{a} & \overline{t^2(4,4)} & \xrightarrow{a} & \overline{ft(0,1)} & \xrightarrow{a} & \overline{t^2(1,4)} & \xrightarrow{a} & \overline{ft(2,1)} \\
 & \xrightarrow{a} & \overline{t^2(3,4)} & \xrightarrow{b} & \overline{ft^2(0,2)} & \xrightarrow{a} & \overline{t(1,3)} & \xrightarrow{a} & \overline{ft^2(2,2)} & \xrightarrow{a} & \overline{t(3,3)} \\
 & \xrightarrow{a} & \overline{ft^2(4,2)} & \xrightarrow{a} & \overline{t(0,3)} & \xrightarrow{a} & \overline{ft^2(1,2)} & \xrightarrow{a} & \overline{t(2,3)} & \xrightarrow{a} & \overline{ft^2(3,2)} \\
 & \xrightarrow{a} & \overline{t(4,3)} & \xrightarrow{b^{-1}} & \overline{f(3,1)} & \xrightarrow{a^{-1}} & \overline{(2,4)} & \xrightarrow{a^{-1}} & \overline{f(1,1)} & \xrightarrow{a^{-1}} & \overline{(0,4)} \\
 & \xrightarrow{a^{-1}} & \overline{f(4,1)} & \xrightarrow{a^{-1}} & \overline{(3,4)} & \xrightarrow{a^{-1}} & \overline{f(2,1)} & \xrightarrow{a^{-1}} & \overline{(1,4)} & \xrightarrow{a^{-1}} & \overline{f(0,1)} \\
 & \xrightarrow{a^{-1}} & \overline{(4,4)} & \xrightarrow{b} & \overline{ft(2,3)} & \xrightarrow{a} & \overline{t^2(3,2)} & \xrightarrow{a} & \overline{ft(4,3)} & \xrightarrow{a} & \overline{t^2(0,2)} \\
 & \xrightarrow{a} & \overline{ft(1,3)} & \xrightarrow{a} & \overline{t^2(2,2)} & \xrightarrow{a} & \overline{ft(3,3)} & \xrightarrow{a} & \overline{t^2(4,2)} & \xrightarrow{a} & \overline{ft(0,3)} \\
 & \xrightarrow{a} & \overline{t^2(1,2)} & \xrightarrow{b} & \overline{ft^2(2,4)} & \xrightarrow{a} & \overline{t(3,1)} & \xrightarrow{a} & \overline{ft^2(4,4)} & \xrightarrow{a} & \overline{t(0,1)} \\
 & \xrightarrow{a} & \overline{ft^2(1,4)} & \xrightarrow{a} & \overline{t(2,1)} & \xrightarrow{a} & \overline{ft^2(3,4)} & \xrightarrow{a} & \overline{t(4,1)} & \xrightarrow{a} & \overline{ft^2(0,4)} \\
 & \xrightarrow{a} & \overline{t(1,1)} & \xrightarrow{b^{-1}} & \overline{f(3,2)} & \xrightarrow{a^{-1}} & \overline{(2,3)} & \xrightarrow{a^{-1}} & \overline{f(1,2)} & \xrightarrow{a^{-1}} & \overline{(0,3)} \\
 & \xrightarrow{a^{-1}} & \overline{f(4,2)} & \xrightarrow{a^{-1}} & \overline{(3,3)} & \xrightarrow{a^{-1}} & \overline{f(2,2)} & \xrightarrow{a^{-1}} & \overline{(1,3)} & \xrightarrow{a^{-1}} & \overline{f(0,2)} \\
 & \xrightarrow{a^{-1}} & \overline{(4,3)} & \xrightarrow{b} & \overline{ft(0,0)} & \xrightarrow{a} & \overline{t^2(1,0)} & \xrightarrow{a} & \overline{ft(2,0)} & \xrightarrow{a} & \overline{t^2(3,0)} \\
 & \xrightarrow{a} & \overline{ft(4,0)} & \xrightarrow{a} & \overline{t^2(0,0)} & \xrightarrow{a} & \overline{ft(1,0)} & \xrightarrow{a} & \overline{t^2(2,0)} & \xrightarrow{a} & \overline{ft(3,0)} \\
 & \xrightarrow{a} & \overline{t^2(4,0)} & \xrightarrow{b} & \overline{ft^2(4,1)} & \xrightarrow{a} & \overline{t(0,4)} & \xrightarrow{a} & \overline{ft^2(1,1)} & \xrightarrow{a} & \overline{t(2,4)} \\
 & \xrightarrow{a} & \overline{ft^2(3,1)} & \xrightarrow{a} & \overline{t(4,4)} & \xrightarrow{a} & \overline{ft^2(0,1)} & \xrightarrow{a} & \overline{t(1,4)} & \xrightarrow{a} & \overline{ft^2(2,1)} \\
 & \xrightarrow{a} & \overline{t(3,4)} & \xrightarrow{b^{-1}} & \overline{f(3,3)} & \xrightarrow{a^{-1}} & \overline{(2,2)} & \xrightarrow{a^{-1}} & \overline{f(1,3)} & \xrightarrow{a^{-1}} & \overline{(0,2)} \\
 & \xrightarrow{a^{-1}} & \overline{f(4,3)} & \xrightarrow{a^{-1}} & \overline{(3,2)} & \xrightarrow{a^{-1}} & \overline{f(2,3)} & \xrightarrow{a^{-1}} & \overline{(1,2)} & \xrightarrow{a^{-1}} & \overline{f(0,3)} \\
 & \xrightarrow{a^{-1}} & \overline{(4,2)} & \xrightarrow{b} & \overline{ft(3,2)} & \xrightarrow{a} & \overline{t^2(4,3)} & \xrightarrow{a} & \overline{ft(0,2)} & \xrightarrow{a} & \overline{t^2(1,3)} \\
 & \xrightarrow{a} & \overline{ft(2,2)} & \xrightarrow{a} & \overline{t^2(3,3)} & \xrightarrow{a} & \overline{ft(4,2)} & \xrightarrow{a} & \overline{t^2(0,3)} & \xrightarrow{a} & \overline{ft(1,2)} \\
 & \xrightarrow{a} & \overline{t^2(2,3)} & \xrightarrow{b} & \overline{ft^2(1,3)} & \xrightarrow{a} & \overline{t(2,2)} & \xrightarrow{a} & \overline{ft^2(3,3)} & \xrightarrow{a} & \overline{t(4,2)} \\
 & \xrightarrow{a} & \overline{ft^2(0,3)} & \xrightarrow{a} & \overline{t(1,2)} & \xrightarrow{a} & \overline{ft^2(2,3)} & \xrightarrow{a} & \overline{t(3,2)} & \xrightarrow{a} & \overline{ft^2(4,3)} \\
 & \xrightarrow{a} & \overline{t(0,2)} & \xrightarrow{b^{-1}} & \overline{f(3,4)} & \xrightarrow{a^{-1}} & \overline{(2,1)} & \xrightarrow{a^{-1}} & \overline{f(1,4)} & \xrightarrow{a^{-1}} & \overline{(0,1)} \\
 & \xrightarrow{a^{-1}} & \overline{f(4,4)} & \xrightarrow{a^{-1}} & \overline{(3,1)} & \xrightarrow{a^{-1}} & \overline{f(2,4)} & \xrightarrow{a^{-1}} & \overline{(1,1)} & \xrightarrow{a^{-1}} & \overline{f(0,4)} \\
 & \xrightarrow{a^{-1}} & \overline{(4,1)} & \xrightarrow{b} & \overline{ft(1,4)} & \xrightarrow{a} & \overline{t^2(2,1)} & \xrightarrow{a} & \overline{ft(3,4)} & \xrightarrow{a} & \overline{t^2(4,1)} \\
 & \xrightarrow{a} & \overline{ft(0,4)} & \xrightarrow{a} & \overline{t^2(1,1)} & \xrightarrow{a} & \overline{ft(2,4)} & \xrightarrow{a} & \overline{t^2(3,1)} & \xrightarrow{a} & \overline{ft(4,4)} \\
 & \xrightarrow{a} & \overline{t^2(0,1)} & \xrightarrow{b} & \overline{ft^2(3,0)} & \xrightarrow{a} & \overline{t(4,0)} & \xrightarrow{a} & \overline{ft^2(0,0)} & \xrightarrow{a} & \overline{t(1,0)} \\
 & \xrightarrow{a} & \overline{ft^2(2,0)} & \xrightarrow{a} & \overline{t(3,0)} & \xrightarrow{a} & \overline{ft^2(4,0)} & \xrightarrow{a} & \overline{t(0,0)} & \xrightarrow{a} & \overline{ft^2(1,0)} \\
 & \xrightarrow{a} & \overline{t(2,0)} & \xrightarrow{b^{-1}} & \overline{f(3,0)} & \xrightarrow{a^{-1}} & \overline{(2,0)} & \xrightarrow{a^{-1}} & \overline{f(1,0)} & \xrightarrow{a^{-1}} & \overline{(0,0)}
\end{array}
$$

$f$ inverts $t$, $t$ is nontrivial on $P$, and $S = \{f(1,0), ft(\lambda, 2\lambda)\}$ with $\lambda = 2$

$$\overline{(0,0)} \xrightarrow{a^{-1}} \overline{f(4,0)} \xrightarrow{a^{-1}} \overline{(3,0)} \xrightarrow{a^{-1}} \overline{f(2,0)} \xrightarrow{a^{-1}} \overline{(1,0)} \xrightarrow{a^{-1}} \overline{f(0,0)}$$
$$\xrightarrow{a^{-1}} \overline{(4,0)} \xrightarrow{b} \overline{ft(0,3)} \xrightarrow{a} \overline{t^2(1,2)} \xrightarrow{a} \overline{ft(2,3)} \xrightarrow{a} \overline{t^2(3,2)}$$
$$\xrightarrow{a} \overline{ft(4,3)} \xrightarrow{a} \overline{t^2(0,2)} \xrightarrow{a} \overline{ft(1,3)} \xrightarrow{a} \overline{t^2(2,2)} \xrightarrow{a} \overline{ft(3,3)}$$
$$\xrightarrow{a} \overline{t^2(4,2)} \xrightarrow{b^{-1}} \overline{ft^2(0,1)} \xrightarrow{a^{-1}} \overline{t(4,4)} \xrightarrow{a^{-1}} \overline{ft^2(3,1)} \xrightarrow{a^{-1}} \overline{t(2,4)}$$
$$\xrightarrow{a^{-1}} \overline{ft^2(1,1)} \xrightarrow{a^{-1}} \overline{t(0,4)} \xrightarrow{a^{-1}} \overline{ft^2(4,1)} \xrightarrow{a^{-1}} \overline{t(3,4)} \xrightarrow{a^{-1}} \overline{ft^2(2,1)}$$
$$\xrightarrow{a^{-1}} \overline{t(1,4)} \xrightarrow{b^{-1}} \overline{f(3,4)} \xrightarrow{a^{-1}} \overline{(2,1)} \xrightarrow{a^{-1}} \overline{f(1,4)} \xrightarrow{a^{-1}} \overline{(0,1)}$$
$$\xrightarrow{a^{-1}} \overline{f(4,4)} \xrightarrow{a^{-1}} \overline{(3,1)} \xrightarrow{a^{-1}} \overline{f(2,4)} \xrightarrow{a^{-1}} \overline{(1,1)} \xrightarrow{a^{-1}} \overline{f(0,4)}$$
$$\xrightarrow{a^{-1}} \overline{(4,1)} \xrightarrow{b} \overline{ft(2,1)} \xrightarrow{a} \overline{t^2(3,4)} \xrightarrow{a} \overline{ft(4,1)} \xrightarrow{a} \overline{t^2(0,4)}$$
$$\xrightarrow{a} \overline{ft(1,1)} \xrightarrow{a} \overline{t^2(2,4)} \xrightarrow{a} \overline{ft(3,1)} \xrightarrow{a} \overline{t^2(4,4)} \xrightarrow{a} \overline{ft(0,1)}$$
$$\xrightarrow{a} \overline{t^2(1,4)} \xrightarrow{b^{-1}} \overline{ft^2(3,4)} \xrightarrow{a^{-1}} \overline{t(2,1)} \xrightarrow{a^{-1}} \overline{ft^2(1,4)} \xrightarrow{a^{-1}} \overline{t(0,1)}$$
$$\xrightarrow{a^{-1}} \overline{ft^2(4,4)} \xrightarrow{a^{-1}} \overline{t(3,1)} \xrightarrow{a^{-1}} \overline{ft^2(2,4)} \xrightarrow{a^{-1}} \overline{t(1,1)} \xrightarrow{a^{-1}} \overline{ft^2(0,4)}$$
$$\xrightarrow{a^{-1}} \overline{t(4,1)} \xrightarrow{b^{-1}} \overline{f(3,3)} \xrightarrow{a^{-1}} \overline{(2,2)} \xrightarrow{a^{-1}} \overline{f(1,3)} \xrightarrow{a^{-1}} \overline{(0,2)}$$
$$\xrightarrow{a^{-1}} \overline{f(4,3)} \xrightarrow{a^{-1}} \overline{(3,2)} \xrightarrow{a^{-1}} \overline{f(2,3)} \xrightarrow{a^{-1}} \overline{(1,2)} \xrightarrow{a^{-1}} \overline{f(0,3)}$$
$$\xrightarrow{a^{-1}} \overline{(4,2)} \xrightarrow{b} \overline{ft(4,4)} \xrightarrow{a} \overline{t^2(0,1)} \xrightarrow{a} \overline{ft(1,4)} \xrightarrow{a} \overline{t^2(2,1)}$$
$$\xrightarrow{a} \overline{ft(3,4)} \xrightarrow{a} \overline{t^2(4,1)} \xrightarrow{a} \overline{ft(0,4)} \xrightarrow{a} \overline{t^2(1,1)} \xrightarrow{a} \overline{ft(2,4)}$$
$$\xrightarrow{a} \overline{t^2(3,1)} \xrightarrow{b^{-1}} \overline{ft^2(1,2)} \xrightarrow{a^{-1}} \overline{t(0,3)} \xrightarrow{a^{-1}} \overline{ft^2(4,2)} \xrightarrow{a^{-1}} \overline{t(3,3)}$$
$$\xrightarrow{a^{-1}} \overline{ft^2(2,2)} \xrightarrow{a^{-1}} \overline{t(1,3)} \xrightarrow{a^{-1}} \overline{ft^2(0,2)} \xrightarrow{a^{-1}} \overline{t(4,3)} \xrightarrow{a^{-1}} \overline{ft^2(3,2)}$$
$$\xrightarrow{a^{-1}} \overline{t(2,3)} \xrightarrow{b^{-1}} \overline{f(3,2)} \xrightarrow{a^{-1}} \overline{(2,3)} \xrightarrow{a^{-1}} \overline{f(1,2)} \xrightarrow{a^{-1}} \overline{(0,3)}$$
$$\xrightarrow{a^{-1}} \overline{f(4,2)} \xrightarrow{a^{-1}} \overline{(3,3)} \xrightarrow{a^{-1}} \overline{f(2,2)} \xrightarrow{a^{-1}} \overline{(1,3)} \xrightarrow{a^{-1}} \overline{f(0,2)}$$
$$\xrightarrow{a^{-1}} \overline{(4,3)} \xrightarrow{b} \overline{ft(1,2)} \xrightarrow{a} \overline{t^2(2,3)} \xrightarrow{a} \overline{ft(3,2)} \xrightarrow{a} \overline{t^2(4,3)}$$
$$\xrightarrow{a} \overline{ft(0,2)} \xrightarrow{a} \overline{t^2(1,3)} \xrightarrow{a} \overline{ft(2,2)} \xrightarrow{a} \overline{t^2(3,3)} \xrightarrow{a} \overline{ft(4,2)}$$
$$\xrightarrow{a} \overline{t^2(0,3)} \xrightarrow{b^{-1}} \overline{ft^2(4,0)} \xrightarrow{a^{-1}} \overline{t(3,0)} \xrightarrow{a^{-1}} \overline{ft^2(2,0)} \xrightarrow{a^{-1}} \overline{t(1,0)}$$
$$\xrightarrow{a^{-1}} \overline{ft^2(0,0)} \xrightarrow{a^{-1}} \overline{t(4,0)} \xrightarrow{a^{-1}} \overline{ft^2(3,0)} \xrightarrow{a^{-1}} \overline{t(2,0)} \xrightarrow{a^{-1}} \overline{ft^2(1,0)}$$
$$\xrightarrow{a^{-1}} \overline{t(0,0)} \xrightarrow{b^{-1}} \overline{f(3,1)} \xrightarrow{a^{-1}} \overline{(2,4)} \xrightarrow{a^{-1}} \overline{f(1,1)} \xrightarrow{a^{-1}} \overline{(0,4)}$$
$$\xrightarrow{a^{-1}} \overline{f(4,1)} \xrightarrow{a^{-1}} \overline{(3,4)} \xrightarrow{a^{-1}} \overline{f(2,1)} \xrightarrow{a^{-1}} \overline{(1,4)} \xrightarrow{a^{-1}} \overline{f(0,1)}$$
$$\xrightarrow{a^{-1}} \overline{(4,4)} \xrightarrow{b} \overline{ft(3,0)} \xrightarrow{a} \overline{t^2(4,0)} \xrightarrow{a} \overline{ft(0,0)} \xrightarrow{a} \overline{t^2(1,0)}$$
$$\xrightarrow{a} \overline{ft(2,0)} \xrightarrow{a} \overline{t^2(3,0)} \xrightarrow{a} \overline{ft(4,0)} \xrightarrow{a} \overline{t^2(0,0)} \xrightarrow{a} \overline{ft(1,0)}$$
$$\xrightarrow{a} \overline{t^2(2,0)} \xrightarrow{b^{-1}} \overline{ft^2(2,3)} \xrightarrow{a^{-1}} \overline{t(1,2)} \xrightarrow{a^{-1}} \overline{ft^2(0,3)} \xrightarrow{a^{-1}} \overline{t(4,2)}$$
$$\xrightarrow{a^{-1}} \overline{ft^2(3,3)} \xrightarrow{a^{-1}} \overline{t(2,2)} \xrightarrow{a^{-1}} \overline{ft^2(1,3)} \xrightarrow{a^{-1}} \overline{t(0,2)} \xrightarrow{a^{-1}} \overline{ft^2(4,3)}$$
$$\xrightarrow{a^{-1}} \overline{t(3,2)} \xrightarrow{b^{-1}} \overline{f(3,0)} \xrightarrow{a^{-1}} \overline{(2,0)} \xrightarrow{a^{-1}} \overline{f(1,0)} \xrightarrow{a^{-1}} \overline{(0,0)}$$

$f$ inverts $t$, $t$ is nontrivial on $P$, and $S = \{f, t, t(1,1)\}$

$$\overline{(0,0)} \xrightarrow{b} \overline{t(0,0)} \xrightarrow{b} \overline{t^2(0,0)} \xrightarrow{a} \overline{ft(0,0)} \xrightarrow{c} \overline{ft^2(1,1)} \xrightarrow{b} \overline{f(0,3)}$$
$$\xrightarrow{a} \overline{(0,2)} \xrightarrow{b} \overline{t(1,4)} \xrightarrow{b} \overline{t^2(4,4)} \xrightarrow{a} \overline{ft(4,1)} \xrightarrow{c} \overline{ft^2(2,2)}$$
$$\xrightarrow{b} \overline{f(0,1)} \xrightarrow{a} \overline{(0,4)} \xrightarrow{b} \overline{t(2,3)} \xrightarrow{b} \overline{t^2(3,3)} \xrightarrow{a} \overline{ft(3,2)}$$
$$\xrightarrow{c} \overline{ft^2(3,3)} \xrightarrow{b^{-1}} \overline{ft(2,3)} \xrightarrow{a} \overline{t^2(2,2)} \xrightarrow{b^{-1}} \overline{t(3,2)} \xrightarrow{b^{-1}} \overline{(0,1)}$$
$$\xrightarrow{a} \overline{f(0,4)} \xrightarrow{c^{-1}} \overline{ft^2(4,2)} \xrightarrow{b} \overline{f(4,3)} \xrightarrow{a} \overline{(4,2)} \xrightarrow{b} \overline{t(4,3)}$$
$$\xrightarrow{b} \overline{t^2(2,0)} \xrightarrow{a} \overline{ft(2,0)} \xrightarrow{c} \overline{ft^2(0,3)} \xrightarrow{b} \overline{f(4,1)} \xrightarrow{a} \overline{(4,4)}$$
$$\xrightarrow{b} \overline{t(0,2)} \xrightarrow{b} \overline{t^2(1,4)} \xrightarrow{a} \overline{ft(1,1)} \xrightarrow{c} \overline{ft^2(1,4)} \xrightarrow{b} \overline{f(4,4)}$$
$$\xrightarrow{a} \overline{(4,1)} \xrightarrow{b} \overline{t(1,1)} \xrightarrow{b} \overline{t^2(0,3)} \xrightarrow{a} \overline{ft(0,2)} \xrightarrow{c} \overline{ft^2(2,0)}$$
$$\xrightarrow{b} \overline{f(4,2)} \xrightarrow{a} \overline{(4,3)} \xrightarrow{b} \overline{t(2,0)} \xrightarrow{b} \overline{t^2(4,2)} \xrightarrow{a} \overline{ft(4,3)}$$
$$\xrightarrow{c} \overline{ft^2(3,1)} \xrightarrow{b^{-1}} \overline{ft(3,4)} \xrightarrow{a} \overline{t^2(3,1)} \xrightarrow{b^{-1}} \overline{t(3,4)} \xrightarrow{b^{-1}} \overline{(4,0)}$$
$$\xrightarrow{a} \overline{f(4,0)} \xrightarrow{c^{-1}} \overline{ft^2(4,0)} \xrightarrow{b} \overline{f(3,4)} \xrightarrow{a} \overline{(3,1)} \xrightarrow{b} \overline{t(4,0)}$$
$$\xrightarrow{b} \overline{t^2(3,4)} \xrightarrow{a} \overline{ft(3,1)} \xrightarrow{c} \overline{ft^2(0,1)} \xrightarrow{b} \overline{f(3,2)} \xrightarrow{a} \overline{(3,3)}$$
$$\xrightarrow{b} \overline{t(0,4)} \xrightarrow{b} \overline{t^2(2,3)} \xrightarrow{a} \overline{ft(2,2)} \xrightarrow{c} \overline{ft^2(1,2)} \xrightarrow{b} \overline{f(3,0)}$$
$$\xrightarrow{a} \overline{(3,0)} \xrightarrow{b} \overline{t(1,3)} \xrightarrow{b} \overline{t^2(1,2)} \xrightarrow{a} \overline{ft(1,3)} \xrightarrow{c} \overline{ft^2(2,3)}$$
$$\xrightarrow{b} \overline{f(3,3)} \xrightarrow{a} \overline{(3,2)} \xrightarrow{b} \overline{t(2,2)} \xrightarrow{b} \overline{t^2(0,1)} \xrightarrow{a} \overline{ft(0,4)}$$
$$\xrightarrow{c} \overline{ft^2(3,4)} \xrightarrow{b^{-1}} \overline{ft(4,0)} \xrightarrow{a} \overline{t^2(4,0)} \xrightarrow{b^{-1}} \overline{t(3,1)} \xrightarrow{b^{-1}} \overline{(3,4)}$$
$$\xrightarrow{a} \overline{f(3,1)} \xrightarrow{c^{-1}} \overline{ft^2(4,3)} \xrightarrow{b} \overline{f(2,0)} \xrightarrow{a} \overline{(2,0)} \xrightarrow{b} \overline{t(4,2)}$$
$$\xrightarrow{b} \overline{t^2(4,3)} \xrightarrow{a} \overline{ft(4,2)} \xrightarrow{c} \overline{ft^2(0,4)} \xrightarrow{b} \overline{f(2,3)} \xrightarrow{a} \overline{(2,2)}$$
$$\xrightarrow{b} \overline{t(0,1)} \xrightarrow{b} \overline{t^2(3,2)} \xrightarrow{a} \overline{ft(3,3)} \xrightarrow{c} \overline{ft^2(1,0)} \xrightarrow{b} \overline{f(2,1)}$$
$$\xrightarrow{a} \overline{(2,4)} \xrightarrow{b} \overline{t(1,0)} \xrightarrow{b} \overline{t^2(2,1)} \xrightarrow{a} \overline{ft(2,4)} \xrightarrow{c} \overline{ft^2(2,1)}$$
$$\xrightarrow{b} \overline{f(2,4)} \xrightarrow{a} \overline{(2,1)} \xrightarrow{b} \overline{t(2,4)} \xrightarrow{b} \overline{t^2(1,0)} \xrightarrow{a} \overline{ft(1,0)}$$
$$\xrightarrow{c} \overline{ft^2(3,2)} \xrightarrow{b^{-1}} \overline{ft(0,1)} \xrightarrow{a} \overline{t^2(0,4)} \xrightarrow{b^{-1}} \overline{t(3,3)} \xrightarrow{b^{-1}} \overline{(2,3)}$$
$$\xrightarrow{a} \overline{f(2,2)} \xrightarrow{c^{-1}} \overline{ft^2(4,1)} \xrightarrow{b} \overline{f(1,1)} \xrightarrow{a} \overline{(1,4)} \xrightarrow{b} \overline{t(4,4)}$$
$$\xrightarrow{b} \overline{t^2(0,2)} \xrightarrow{a} \overline{ft(0,3)} \xrightarrow{c} \overline{ft^2(0,2)} \xrightarrow{b} \overline{f(1,4)} \xrightarrow{a} \overline{(1,1)}$$
$$\xrightarrow{b} \overline{t(0,3)} \xrightarrow{b} \overline{t^2(4,1)} \xrightarrow{a} \overline{ft(4,4)} \xrightarrow{c} \overline{ft^2(1,3)} \xrightarrow{b} \overline{f(1,2)}$$
$$\xrightarrow{a} \overline{(1,3)} \xrightarrow{b} \overline{t(1,2)} \xrightarrow{b} \overline{t^2(3,0)} \xrightarrow{a} \overline{ft(3,0)} \xrightarrow{c} \overline{ft^2(2,4)}$$
$$\xrightarrow{b} \overline{f(1,0)} \xrightarrow{a} \overline{(1,0)} \xrightarrow{b} \overline{t(2,1)} \xrightarrow{b} \overline{t^2(2,4)} \xrightarrow{a} \overline{ft(2,1)}$$
$$\xrightarrow{c} \overline{ft^2(3,0)} \xrightarrow{b^{-1}} \overline{ft(1,2)} \xrightarrow{a} \overline{t^2(1,3)} \xrightarrow{b^{-1}} \overline{t(3,0)} \xrightarrow{b^{-1}} \overline{(1,2)}$$
$$\xrightarrow{a} \overline{f(1,3)} \xrightarrow{c^{-1}} \overline{ft^2(4,4)} \xrightarrow{b} \overline{f(0,2)} \xrightarrow{a} \overline{(0,3)} \xrightarrow{b} \overline{t(4,1)}$$
$$\xrightarrow{b} \overline{t^2(1,1)} \xrightarrow{a} \overline{ft(1,4)} \xrightarrow{c} \overline{ft^2(0,0)} \xrightarrow{b} \overline{f(0,0)} \xrightarrow{a} \overline{(0,0)}$$

$f$ inverts $t$, $t$ is nontrivial on $P$, and $S = \{f, ft, f(0,1)\}$

$$
\begin{array}{ccccccccccc}
\overline{(0,0)} & \xrightarrow{b} & \overline{ft(0,0)} & \xrightarrow{c} & \overline{t^2(0,1)} & \xrightarrow{b} & \overline{ft^2(2,3)} & \xrightarrow{a} & \overline{t(2,2)} & \xrightarrow{b} & \overline{f(3,3)} \\
 & \xrightarrow{a} & \overline{(3,2)} & \xrightarrow{b} & \overline{ft(0,4)} & \xrightarrow{c} & \overline{t^2(0,2)} & \xrightarrow{b} & \overline{ft^2(4,1)} & \xrightarrow{c} & \overline{t(4,0)} \\
 & \xrightarrow{b} & \overline{f(3,4)} & \xrightarrow{a} & \overline{(3,1)} & \xrightarrow{b} & \overline{ft(3,1)} & \xrightarrow{c} & \overline{t^2(3,0)} & \xrightarrow{b} & \overline{ft^2(1,3)} \\
 & \xrightarrow{a} & \overline{t(1,2)} & \xrightarrow{b} & \overline{f(1,2)} & \xrightarrow{a} & \overline{(1,3)} & \xrightarrow{b} & \overline{ft(3,0)} & \xrightarrow{c} & \overline{t^2(3,1)} \\
 & \xrightarrow{b} & \overline{ft^2(3,1)} & \xrightarrow{a} & \overline{t(3,4)} & \xrightarrow{b} & \overline{f(4,0)} & \xrightarrow{a} & \overline{(4,0)} & \xrightarrow{b} & \overline{ft(3,4)} \\
 & \xrightarrow{c} & \overline{t^2(3,2)} & \xrightarrow{b} & \overline{ft^2(0,4)} & \xrightarrow{a} & \overline{t(0,1)} & \xrightarrow{b} & \overline{f(2,3)} & \xrightarrow{a} & \overline{(2,2)} \\
 & \xrightarrow{b} & \overline{ft(3,3)} & \xrightarrow{c} & \overline{t^2(3,3)} & \xrightarrow{b} & \overline{ft^2(2,2)} & \xrightarrow{a} & \overline{t(2,3)} & \xrightarrow{b} & \overline{f(0,1)} \\
 & \xrightarrow{a} & \overline{(0,4)} & \xrightarrow{b} & \overline{ft(3,2)} & \xrightarrow{c} & \overline{t^2(3,4)} & \xrightarrow{b} & \overline{ft^2(4,0)} & \xrightarrow{c} & \overline{t(4,1)} \\
 & \xrightarrow{b} & \overline{f(0,2)} & \xrightarrow{a} & \overline{(0,3)} & \xrightarrow{b} & \overline{ft(1,4)} & \xrightarrow{c} & \overline{t^2(1,2)} & \xrightarrow{b} & \overline{ft^2(1,2)} \\
 & \xrightarrow{a} & \overline{t(1,3)} & \xrightarrow{b} & \overline{f(3,0)} & \xrightarrow{a} & \overline{(3,0)} & \xrightarrow{b} & \overline{ft(1,3)} & \xrightarrow{c} & \overline{t^2(1,3)} \\
 & \xrightarrow{b} & \overline{ft^2(3,0)} & \xrightarrow{a} & \overline{t(3,0)} & \xrightarrow{b} & \overline{f(1,3)} & \xrightarrow{a} & \overline{(1,2)} & \xrightarrow{b} & \overline{ft(1,2)} \\
 & \xrightarrow{c} & \overline{t^2(1,4)} & \xrightarrow{b} & \overline{ft^2(0,3)} & \xrightarrow{a} & \overline{t(0,2)} & \xrightarrow{b} & \overline{f(4,1)} & \xrightarrow{a} & \overline{(4,4)} \\
 & \xrightarrow{b} & \overline{ft(1,1)} & \xrightarrow{c} & \overline{t^2(1,0)} & \xrightarrow{b} & \overline{ft^2(2,1)} & \xrightarrow{a} & \overline{t(2,4)} & \xrightarrow{b} & \overline{f(2,4)} \\
 & \xrightarrow{a} & \overline{(2,1)} & \xrightarrow{b} & \overline{ft(1,0)} & \xrightarrow{c} & \overline{t^2(1,1)} & \xrightarrow{b} & \overline{ft^2(4,4)} & \xrightarrow{c} & \overline{t(4,2)} \\
 & \xrightarrow{b} & \overline{f(2,0)} & \xrightarrow{a} & \overline{(2,0)} & \xrightarrow{b} & \overline{ft(4,2)} & \xrightarrow{c} & \overline{t^2(4,4)} & \xrightarrow{b} & \overline{ft^2(1,1)} \\
 & \xrightarrow{a} & \overline{t(1,4)} & \xrightarrow{b} & \overline{f(0,3)} & \xrightarrow{a} & \overline{(0,2)} & \xrightarrow{b} & \overline{ft(4,1)} & \xrightarrow{c} & \overline{t^2(4,0)} \\
 & \xrightarrow{b} & \overline{ft^2(3,4)} & \xrightarrow{a} & \overline{t(3,1)} & \xrightarrow{b} & \overline{f(3,1)} & \xrightarrow{a} & \overline{(3,4)} & \xrightarrow{b} & \overline{ft(4,0)} \\
 & \xrightarrow{c} & \overline{t^2(4,1)} & \xrightarrow{b} & \overline{ft^2(0,2)} & \xrightarrow{a} & \overline{t(0,3)} & \xrightarrow{b} & \overline{f(1,4)} & \xrightarrow{a} & \overline{(1,1)} \\
 & \xrightarrow{b} & \overline{ft(4,4)} & \xrightarrow{c} & \overline{t^2(4,2)} & \xrightarrow{b} & \overline{ft^2(2,0)} & \xrightarrow{a} & \overline{t(2,0)} & \xrightarrow{b} & \overline{f(4,2)} \\
 & \xrightarrow{a} & \overline{(4,3)} & \xrightarrow{b} & \overline{ft(4,3)} & \xrightarrow{c} & \overline{t^2(4,3)} & \xrightarrow{b} & \overline{ft^2(4,3)} & \xrightarrow{c} & \overline{t(4,3)} \\
 & \xrightarrow{b} & \overline{f(4,3)} & \xrightarrow{a} & \overline{(4,2)} & \xrightarrow{b} & \overline{ft(2,0)} & \xrightarrow{c} & \overline{t^2(2,1)} & \xrightarrow{b} & \overline{ft^2(1,0)} \\
 & \xrightarrow{a} & \overline{t(1,0)} & \xrightarrow{b} & \overline{f(2,1)} & \xrightarrow{a} & \overline{(2,4)} & \xrightarrow{b} & \overline{ft(2,4)} & \xrightarrow{c} & \overline{t^2(2,2)} \\
 & \xrightarrow{b} & \overline{ft^2(3,3)} & \xrightarrow{a} & \overline{t(3,2)} & \xrightarrow{b} & \overline{f(0,4)} & \xrightarrow{a} & \overline{(0,1)} & \xrightarrow{b} & \overline{ft(2,3)} \\
 & \xrightarrow{c} & \overline{t^2(2,3)} & \xrightarrow{b} & \overline{ft^2(0,1)} & \xrightarrow{a} & \overline{t(0,4)} & \xrightarrow{b} & \overline{f(3,2)} & \xrightarrow{a} & \overline{(3,3)} \\
 & \xrightarrow{b} & \overline{ft(2,2)} & \xrightarrow{c} & \overline{t^2(2,4)} & \xrightarrow{b} & \overline{ft^2(2,4)} & \xrightarrow{a} & \overline{t(2,1)} & \xrightarrow{b} & \overline{f(1,0)} \\
 & \xrightarrow{a} & \overline{(1,0)} & \xrightarrow{b} & \overline{ft(2,1)} & \xrightarrow{c} & \overline{t^2(2,0)} & \xrightarrow{b} & \overline{ft^2(4,2)} & \xrightarrow{c} & \overline{t(4,4)} \\
 & \xrightarrow{b} & \overline{f(1,1)} & \xrightarrow{a} & \overline{(1,4)} & \xrightarrow{b} & \overline{ft(0,3)} & \xrightarrow{c} & \overline{t^2(0,3)} & \xrightarrow{b} & \overline{ft^2(1,4)} \\
 & \xrightarrow{a} & \overline{t(1,1)} & \xrightarrow{b} & \overline{f(4,4)} & \xrightarrow{a} & \overline{(4,1)} & \xrightarrow{b} & \overline{ft(0,2)} & \xrightarrow{c} & \overline{t^2(0,4)} \\
 & \xrightarrow{b} & \overline{ft^2(3,2)} & \xrightarrow{a} & \overline{t(3,3)} & \xrightarrow{b} & \overline{f(2,2)} & \xrightarrow{a} & \overline{(2,3)} & \xrightarrow{b} & \overline{ft(0,1)} \\
 & \xrightarrow{c} & \overline{t^2(0,0)} & \xrightarrow{b} & \overline{ft^2(0,0)} & \xrightarrow{a} & \overline{t(0,0)} & \xrightarrow{b} & \overline{f(0,0)} & \xrightarrow{a} & \overline{(0,0)}
\end{array}
$$

$f$ inverts $t$, $t$ is nontrivial on $P$, and $S = \{f, ft, ft^2(1,-1)\}$

$$\overline{(0,0)} \xrightarrow{c} \overline{ft^2(1,4)} \xrightarrow{b} \overline{t^2(0,3)} \xrightarrow{a} \overline{ft(0,2)} \xrightarrow{c} \overline{t(2,0)} \xrightarrow{b} \overline{f(4,2)}$$
$$\xrightarrow{a} \overline{(4,3)} \xrightarrow{c} \overline{ft^2(3,4)} \xrightarrow{b} \overline{t^2(4,0)} \xrightarrow{a} \overline{ft(4,0)} \xrightarrow{b} \overline{(3,4)}$$
$$\xrightarrow{a} \overline{f(3,1)} \xrightarrow{b} \overline{t(3,1)} \xrightarrow{c} \overline{ft(0,4)} \xrightarrow{a} \overline{t^2(0,1)} \xrightarrow{b} \overline{ft^2(2,3)}$$
$$\xrightarrow{c} \overline{(4,1)} \xrightarrow{a} \overline{f(4,4)} \xrightarrow{b} \overline{t(1,1)} \xrightarrow{c} \overline{ft(1,1)} \xrightarrow{a} \overline{t^2(1,4)}$$
$$\xrightarrow{b} \overline{ft^2(0,3)} \xrightarrow{c} \overline{(0,3)} \xrightarrow{a} \overline{f(0,2)} \xrightarrow{c} \overline{t^2(2,0)} \xrightarrow{b} \overline{ft^2(4,2)}$$
$$\xrightarrow{c} \overline{(0,1)} \xrightarrow{a} \overline{f(0,4)} \xrightarrow{b} \overline{t(3,2)} \xrightarrow{c} \overline{ft(3,2)} \xrightarrow{a} \overline{t^2(3,3)}$$
$$\xrightarrow{b} \overline{ft^2(2,2)} \xrightarrow{c} \overline{(1,3)} \xrightarrow{a} \overline{f(1,2)} \xrightarrow{b} \overline{t(1,2)} \xrightarrow{c} \overline{ft(4,4)}$$
$$\xrightarrow{a} \overline{t^2(4,1)} \xrightarrow{b} \overline{ft^2(0,2)} \xrightarrow{c} \overline{(2,0)} \xrightarrow{a} \overline{f(2,0)} \xrightarrow{c} \overline{t^2(0,2)}$$
$$\xrightarrow{a} \overline{ft(0,3)} \xrightarrow{c} \overline{t(0,3)} \xrightarrow{b} \overline{f(1,4)} \xrightarrow{a} \overline{(1,1)} \xrightarrow{c} \overline{ft^2(1,1)}$$
$$\xrightarrow{b} \overline{t^2(4,4)} \xrightarrow{a} \overline{ft(4,1)} \xrightarrow{c} \overline{t(2,3)} \xrightarrow{b} \overline{f(0,1)} \xrightarrow{a} \overline{(0,4)}$$
$$\xrightarrow{c} \overline{ft^2(3,1)} \xrightarrow{b} \overline{t^2(3,1)} \xrightarrow{a} \overline{ft(3,4)} \xrightarrow{c} \overline{t(4,3)} \xrightarrow{b} \overline{f(4,3)}$$
$$\xrightarrow{c} \overline{t^2(3,4)} \xrightarrow{a} \overline{ft(3,1)} \xrightarrow{c} \overline{t(0,4)} \xrightarrow{b} \overline{f(3,2)} \xrightarrow{a} \overline{(3,3)}$$
$$\xrightarrow{c} \overline{ft^2(1,0)} \xrightarrow{b} \overline{t^2(2,1)} \xrightarrow{a} \overline{ft(2,4)} \xrightarrow{c} \overline{t(2,4)} \xrightarrow{b} \overline{f(2,4)}$$
$$\xrightarrow{a} \overline{(2,1)} \xrightarrow{c} \overline{ft^2(3,0)} \xrightarrow{b} \overline{t^2(1,3)} \xrightarrow{a} \overline{ft(1,2)} \xrightarrow{c} \overline{t(4,4)}$$
$$\xrightarrow{a} \overline{ft^2(4,1)} \xrightarrow{c} \overline{(2,3)} \xrightarrow{a} \overline{f(2,2)} \xrightarrow{b} \overline{t(3,3)} \xrightarrow{c} \overline{ft(1,0)}$$
$$\xrightarrow{a} \overline{t^2(1,0)} \xrightarrow{b} \overline{ft^2(2,1)} \xrightarrow{c} \overline{(3,0)} \xrightarrow{a} \overline{f(3,0)} \xrightarrow{b} \overline{t(1,3)}$$
$$\xrightarrow{c} \overline{ft(2,2)} \xrightarrow{a} \overline{t^2(2,3)} \xrightarrow{b} \overline{ft^2(0,1)} \xrightarrow{c} \overline{(4,2)} \xrightarrow{b} \overline{ft(2,0)}$$
$$\xrightarrow{c} \overline{t(0,2)} \xrightarrow{b} \overline{f(4,1)} \xrightarrow{a} \overline{(4,4)} \xrightarrow{c} \overline{ft^2(1,2)} \xrightarrow{b} \overline{t^2(1,2)}$$
$$\xrightarrow{a} \overline{ft(1,3)} \xrightarrow{c} \overline{t(2,2)} \xrightarrow{b} \overline{f(3,3)} \xrightarrow{a} \overline{(3,2)} \xrightarrow{c} \overline{ft^2(3,2)}$$
$$\xrightarrow{b} \overline{t^2(0,4)} \xrightarrow{a} \overline{ft(0,1)} \xrightarrow{c} \overline{t(4,2)} \xrightarrow{a} \overline{ft^2(4,3)} \xrightarrow{b} \overline{t^2(4,3)}$$
$$\xrightarrow{a} \overline{ft(4,2)} \xrightarrow{c} \overline{t(0,1)} \xrightarrow{b} \overline{f(2,3)} \xrightarrow{a} \overline{(2,2)} \xrightarrow{c} \overline{ft^2(1,3)}$$
$$\xrightarrow{b} \overline{t^2(3,0)} \xrightarrow{a} \overline{ft(3,0)} \xrightarrow{c} \overline{t(2,1)} \xrightarrow{b} \overline{f(1,0)} \xrightarrow{a} \overline{(1,0)}$$
$$\xrightarrow{c} \overline{ft^2(3,3)} \xrightarrow{b} \overline{t^2(2,2)} \xrightarrow{a} \overline{ft(2,3)} \xrightarrow{c} \overline{t(4,1)} \xrightarrow{a} \overline{ft^2(4,4)}$$
$$\xrightarrow{c} \overline{(1,2)} \xrightarrow{a} \overline{f(1,3)} \xrightarrow{b} \overline{t(3,0)} \xrightarrow{c} \overline{ft(2,1)} \xrightarrow{a} \overline{t^2(2,4)}$$
$$\xrightarrow{b} \overline{ft^2(2,4)} \xrightarrow{c} \overline{(2,4)} \xrightarrow{a} \overline{f(2,1)} \xrightarrow{b} \overline{t(1,0)} \xrightarrow{c} \overline{ft(3,3)}$$
$$\xrightarrow{a} \overline{t^2(3,2)} \xrightarrow{b} \overline{ft^2(0,4)} \xrightarrow{c} \overline{(3,1)} \xrightarrow{a} \overline{f(3,4)} \xrightarrow{b} \overline{t(4,0)}$$
$$\xrightarrow{a} \overline{ft^2(4,0)} \xrightarrow{c} \overline{(4,0)} \xrightarrow{a} \overline{f(4,0)} \xrightarrow{b} \overline{t(3,4)} \xrightarrow{c} \overline{ft(4,3)}$$
$$\xrightarrow{a} \overline{t^2(4,2)} \xrightarrow{b} \overline{ft^2(2,0)} \xrightarrow{c} \overline{(0,2)} \xrightarrow{a} \overline{f(0,3)} \xrightarrow{b} \overline{t(1,4)}$$
$$\xrightarrow{c} \overline{ft(0,0)} \xrightarrow{a} \overline{t^2(0,0)} \xrightarrow{b} \overline{ft^2(0,0)} \xrightarrow{c} \overline{(1,4)} \xrightarrow{a} \overline{f(1,1)}$$
$$\xrightarrow{c} \overline{t^2(1,1)} \xrightarrow{a} \overline{ft(1,4)} \xrightarrow{c} \overline{t(0,0)} \xrightarrow{b} \overline{f(0,0)} \xrightarrow{a} \overline{(0,0)}$$

## Additional references

[15] B. Alspach and C. Q. Zhang: Hamilton cycles in cubic Cayley graphs on dihedral groups. *Ars Combinatoria* 28 (1989), 101–108.

[16] E. Ghaderpour and D. W. Morris: Cayley graphs of order $30p$ are hamiltonian (preprint). http://arxiv.org/abs/1102.5156

Department of Mathematics and Computer Science, University of Lethbridge, Lethbridge, Alberta, T1K 3M4, Canada

Department of Mathematics and Computer Science, University of Lethbridge, Lethbridge, Alberta, T1K 3M4, Canada
